# Supplementary material for: SparseP: Towards Efficient Sparse Matrix Vector Multiplication on Real Processing-In-Memory Systems
Source: arXiv:2201.05072 source file (2022-05-23)
Supplement: Supplementary file 1 [file 10-appendix.tex]

\section*{{\Large APPENDIX}}
\appendix

\section{Extended Results}

\begin{comment}
\subsection{Load Balancing Techniques among Tasklets of One DPU}\label{sec:appendix-1DPU-Balance}
Figure~\ref{fig:1DPU-datatypes-appendix} provides a complete evaluation for all matrices of our small dataset presented in Section~\ref{1DPU}, i.e., to compare load balancing schemes among tasklets of a DPU for each particular compressed matrix format. The reported key observations of Section~\ref{1DPU} apply to all matrices with diverse sparsity patterns.



\begin{figure}[H]
\vspace{-8pt}
\centering
\begin{minipage}{\textwidth}
\includegraphics[width=.245\textwidth]{1DPU/csr_datatypes_delaunay-n13_16.pdf}
\includegraphics[width=.245\textwidth]{1DPU/csr_datatypes_wing-nodal_16.pdf}
\includegraphics[width=.245\textwidth]{1DPU/csr_datatypes_raefsky4_16.pdf}
\includegraphics[width=.245\textwidth]{1DPU/csr_datatypes_pkustk08_16.pdf}
\end{minipage}\hspace{2pt}%
\begin{minipage}{\textwidth}
\includegraphics[width=.245\textwidth]{1DPU/coo_datatypes_delaunay-n13_16.pdf}
\includegraphics[width=.245\textwidth]{1DPU/coo_datatypes_wing-nodal_16.pdf}
\includegraphics[width=.245\textwidth]{1DPU/coo_datatypes_raefsky4_16.pdf}
\includegraphics[width=.245\textwidth]{1DPU/coo_datatypes_pkustk08_16.pdf}
\end{minipage}\hspace{2pt}%
\begin{minipage}{\textwidth}
\includegraphics[width=.245\textwidth]{1DPU/bcsr_datatypes_delaunay-n13_16.pdf}
\includegraphics[width=.245\textwidth]{1DPU/bcsr_datatypes_wing-nodal_16.pdf}
\includegraphics[width=.245\textwidth]{1DPU/bcsr_datatypes_raefsky4_16.pdf}
\includegraphics[width=.245\textwidth]{1DPU/bcsr_datatypes_pkustk08_16.pdf}
\end{minipage}\hspace{2pt}%
\begin{minipage}{\textwidth}
\includegraphics[width=.245\textwidth]{1DPU/bcoo_datatypes_delaunay-n13_16.pdf}
\includegraphics[width=.245\textwidth]{1DPU/bcoo_datatypes_wing-nodal_16.pdf}
\includegraphics[width=.245\textwidth]{1DPU/bcoo_datatypes_raefsky4_16.pdf}
\includegraphics[width=.245\textwidth]{1DPU/bcoo_datatypes_pkustk08_16.pdf}
\end{minipage}
\vspace{-8pt}
\caption{Performance achieved using 16 tasklets for all data types and compressed matrix formats.}
\label{fig:1DPU-datatypes-appendix}
\vspace{-14pt}
\end{figure}
\end{comment}

\subsection{Synchronization Approaches in Block Formats}\label{sec:appendix-1DPU-BCOO}

We compare the coarse-grain locking and the fine-grain locking approaches in BCOO format. Figure~\ref{fig:1DPU-bcoo-balance} shows the performance achieved by BCOO for all data types and small matrices using 16 tasklets of one DPU. We evaluate all small matrices of Table~\ref{tab:small-matrices}: delaunay\_n13 (\textbf{D}), wing\_nodal (\textbf{W}), raefsky4 (\textbf{R}) and pkustk08 (\textbf{P}).



\begin{figure}[H]
    \vspace{-8pt}
    \centering
    \includegraphics[width=\textwidth]{1DPU/bcoo_locking_kernel_tasklets16.pdf}
    \vspace{-14pt}
    \caption{Performance of BCOO format for all data types and small matrices using 16 tasklets of one DPU.}
    \label{fig:1DPU-bcoo-balance}
    \vspace{-8pt}
\end{figure}


Our key finding is that the fine-grain locking scheme performs similarly with the coarse-grain locking scheme. The fine-grain locking scheme does not increase parallelism in UPMEM PIM architecture, since by default all memory accesses to a DRAM bank are serialized in the DMA engine, thus critical sections are serialized. The same finding holds for all formats.



%\subsection{Evaluation of NNZ vs Block partitioning on RBDBCOO and BDBCOO implementations}
%\subsection{YINIT host vs YINIT DPU in COO format}

\subsection{Fine-grain Data Transfers in 2D Partitioning}\label{sec:appendix-2D-fgtrans}
Figures ~\ref{fig:2D_vp2_fgtransfers} and ~\ref{fig:2D_vp32_fgtransfers} show the performance comparison between coarse-grain and fine-grain data transfers (presented in Section~\ref{2D-FineGrainTransfers}) for all matrices of our large matrix dataset. The reported key findings of Section~\ref{2D-FineGrainTransfers} apply to all matrices with diverse sparsity patterns.



\begin{figure}[H]
    \vspace{-12pt}
    \centering
    \includegraphics[width=1\textwidth]{2D-partitioning/trans_dpus2048_int32_cps2.pdf}
    \vspace{-24pt}
    \caption{Performance comparison of RC: rbdcoo with coarse-grain transfers, RY: rbdcoo with fine-grain transfers in the output vector, BC: bdcoo with coarse-grain transfers, BY: bdcoo with fine-grain transfers only in the output vector, and BT: bdcoo with fine-grain transfers in both the input and the output vector using int32 data type, 2048 DPUs and having 2 vertical partitions.}
    \label{fig:2D_vp2_fgtransfers}
    \vspace{-14pt}
\end{figure}

\begin{figure}[H]
    \vspace{-12pt}
    \centering
    \includegraphics[width=1\textwidth]{2D-partitioning/trans_dpus2048_int32_cps32.pdf}
    \vspace{-24pt}
    \caption{Performance comparison of RC: rbdcoo with coarse-grain transfers, RY: rbdcoo with fine-grain transfers in the output vector, BC: bdcoo with coarse-grain transfers, BY: bdcoo with fine-grain transfers only in the output vector, and BT: bdcoo with fine-grain transfers in both the input and the output vector using int32 data type, 2048 DPUs and having 32 vertical partitions.}
    \label{fig:2D_vp32_fgtransfers}
    \vspace{-14pt}
\end{figure}



\subsection{End-to-end Performance Characterization of 2D Partitioning Techniques}\label{sec:appendix-2D-formats}
Figures~\ref{fig:2D_formats_fixed_all},~\ref{fig:2D_formats_rbal_all},~\ref{fig:2D_formats_bal_all} show the performance comparison between various compression formats (presented in Section~\ref{2D-EndToEnd}) for all matrices of our large matrix dataset. We make two key observations. First, in \equallySized{} techniques, the kernel time in scale-free matrices constitutes a higher portion of the total time compared to regular matrices, since it is bottlenecked by the DPU that processes a much higher number of non-zero elements over the rest. Second, we find that CSR and BCSR perform worse than COO and BCOO, especially in \equallyWidth{} and \variableSized{} schemes, since their data partitioning is limited by row and block-row granularity, respectively, thus they incur higher non-zero imbalance among tasklets of a DPU and among DPUs compared to COO and BCOO formats.


\begin{figure}[H]
    \vspace{-10pt}
    \centering
    \includegraphics[width=1\textwidth]{2D-partitioning/fixed_time_dpus2048_int32_cps4.pdf}
    \vspace{-24pt}
    \caption{End-to-end time breakdown of \equallySized{} 2D partitioning kernels for CR: CSR, CO: COO, BR: BCSR and BO: BCOO formats using 4 vertical partitions and int32 data type.}
    \label{fig:2D_formats_fixed_all}
    \vspace{-8pt}
\end{figure}


\begin{figure}[H]
    \vspace{-10pt}
    \centering
    \includegraphics[width=1\textwidth]{2D-partitioning/rbal_time_dpus2048_int32_cps4.pdf}
    \vspace{-24pt}
    \caption{End-to-end time breakdown of \equallyWidth{} 2D partitioning kernels for CR: CSR, CO: COO, BR: BCSR and BO: BCOO formats using 4 vertical partitions and int32 data type.}
    \label{fig:2D_formats_rbal_all}
    \vspace{-8pt}
\end{figure}

\begin{figure}[H]
    \vspace{-10pt}
    \centering
    \includegraphics[width=1\textwidth]{2D-partitioning/bal_time_dpus2048_int32_cps4.pdf}
    \vspace{-24pt}
    \caption{End-to-end time breakdown of \variableSized{} 2D partitioning kernels for CR: CSR, CO: COO, BR: BCSR and BO: BCOO formats using 4 vertical partitions and int32 data type.}
    \label{fig:2D_formats_bal_all}
    \vspace{-8pt}
\end{figure}



\begin{comment}
\subsection{Scalability of 2D Partitioning Techniques}\label{sec:appendix-2D-scale}
Figures~\ref{fig:2D_scale_four_parittions} and ~\ref{fig:2D_scale_sixteen_parittions}  present a scalability analysis to the number of DPUs for the 2D partitioning techniques using the COO format and having 4 and 16 vertical partitions, respectively. We make two observations. 


\begin{figure}[H]
    \vspace{-6pt}
    \centering
    \begin{minipage}{\textwidth}
    \includegraphics[width=.33\textwidth]{2D-partitioning/scalability_fix_int32_col4.pdf}
    \includegraphics[width=.33\textwidth]{2D-partitioning/scalability_rbal_int32_col4.pdf}
    \includegraphics[width=.33\textwidth]{2D-partitioning/scalability_bal_int32_col4.pdf}
    \end{minipage}
    \vspace{-10pt}
    \caption{Time breakdown of \equallySized{}, \equallyWidth{} and \variableSized{} partitioning techniques using COO format and 4 vertical partitions when varying the number of DPUs used for int32 data type.}
    \label{fig:2D_scale_four_parittions}
    \vspace{-6pt}
\end{figure}


\begin{figure}[H]
    \vspace{-6pt}
    \centering
    \begin{minipage}{\textwidth}
    \includegraphics[width=.33\textwidth]{2D-partitioning/scalability_fix_int32_col16.pdf}
    \includegraphics[width=.33\textwidth]{2D-partitioning/scalability_rbal_int32_col16.pdf}
    \includegraphics[width=.33\textwidth]{2D-partitioning/scalability_bal_int32_col16.pdf}
    \end{minipage}
    \vspace{-10pt}
    \caption{Time breakdown of \equallySized{}, \equallyWidth{} and \variableSized{} partitioning techniques using COO format and 16 vertical partitions when varying the number of DPUs used for int32 data type.}
    \label{fig:2D_scale_sixteen_parittions}
    \vspace{-6pt}
\end{figure}

First, the \equallySized{} scheme achieves high scalability with a high number of vertical partitions. With a high number of vertical partitions the non-zero element deviation among DPUs is high, i.e., the kernel time is bottleneck by the DPU that processes the highest number of non-zero elements, thus increasing the number of DPUs improves performance by decreasing the kernel time. Instead, with a smaller number of vertical partitions \equallySized{} scheme scales as the number of DPU increases, mainly in \textit{scale-free} matrices (e.g., sxw and ask matrices), where there is high non-zero element deviation among DPUs due to their highly irregular pattern. Second, we observe that the \equallyWidth{} and \variableSized{} schemes are severely bottlenecked by retrieve data transfer costs (a high amount of padding is needed for parallel transfers), thus they do typically not scale as the number of DPUs increases. Moreover, when the number of vertical partitions is higher, the deviation on the heights of the tiles is higher, thus as the number of DPUs increases the amount of padding needed in retrieve data transfers increases with a higher rate, which in turn severely degrades performance.

\end{comment}


\subsection{Arithmetic Throughput of a DPU}\label{sec:appendix-1DPU-AT}
%\subsubsection{Microbenchmark Description.}
We evaluate the arithmetic throughput of the DPU for MUL operation. We use a microbenchmark from PrIM~\cite{Gomez2021Benchmarking} and configure it for all data types. Figure~\ref{fig:1DPU-ai} shows how the measured arithmetic throughput (in MOPS) for the multiplication (MUL) operation on one DPU varies with the number of tasklets for all data types. The arithmetic throughput for MUL operations is 12.94MOps, 10.52MOps, 8.86MOps, 2.84MOps, 1.84MOps, and 0.51MOps for int8, int16, int32, int64, flt32 and dbl64 data types, respectively.



\begin{figure}[H]
\centering
\vspace{-12pt}
\begin{minipage}{1.03\textwidth}
%\centering
\includegraphics[width=.3\textwidth]{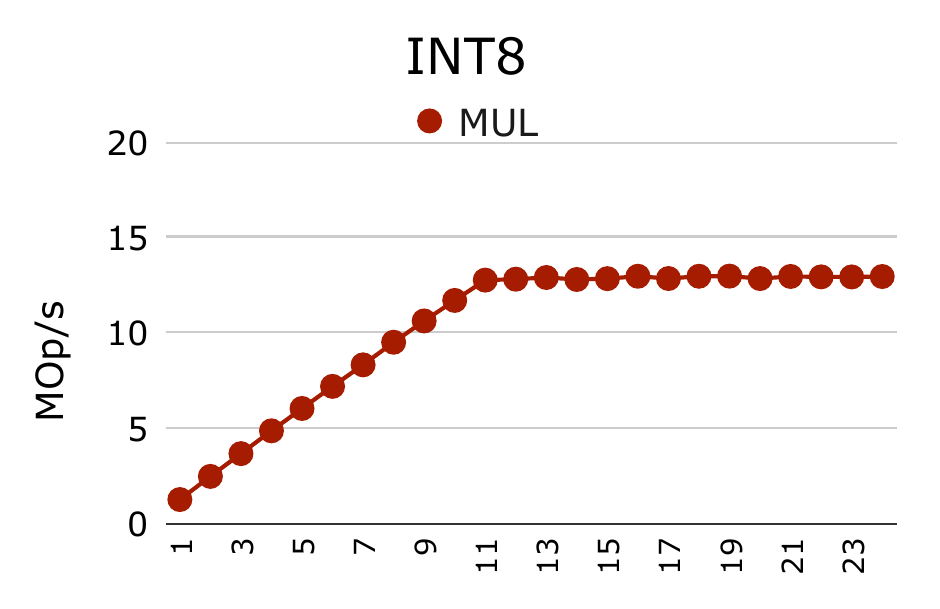} \hspace{4pt}
\includegraphics[width=.3\textwidth]{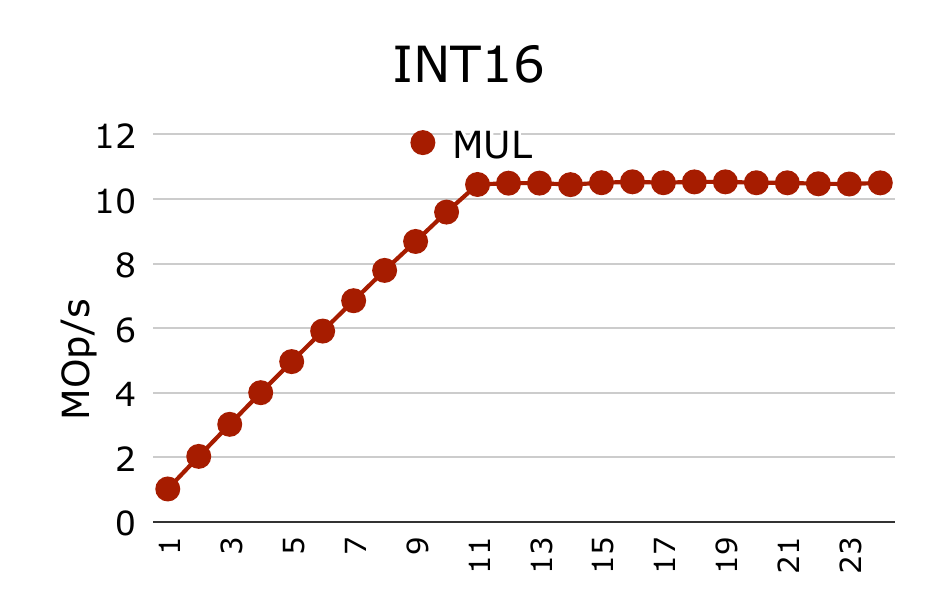}\hspace{4pt}
\includegraphics[width=.3\textwidth]{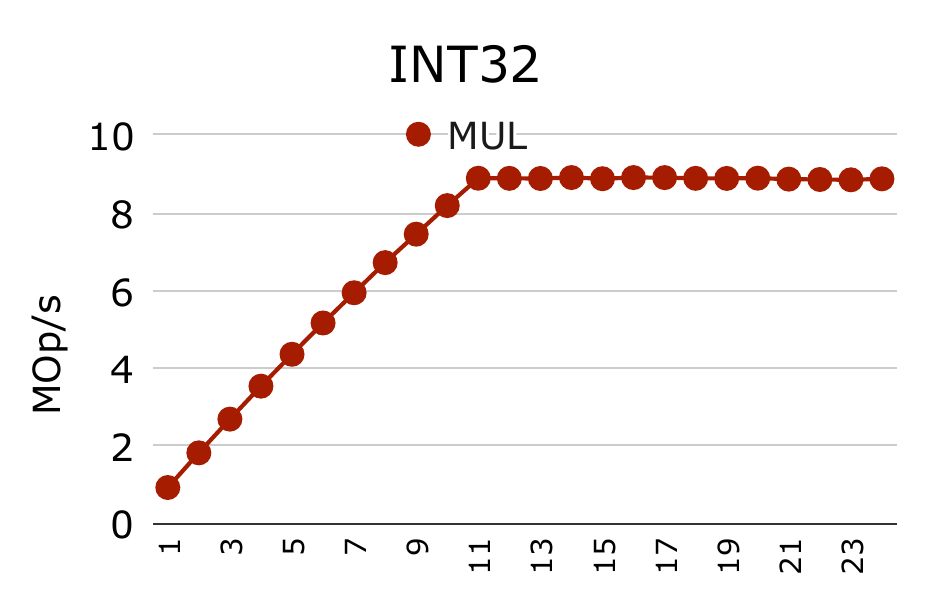}
\end{minipage} % 
\begin{minipage}{1.03\textwidth}
%\centering
\includegraphics[width=.3\textwidth]{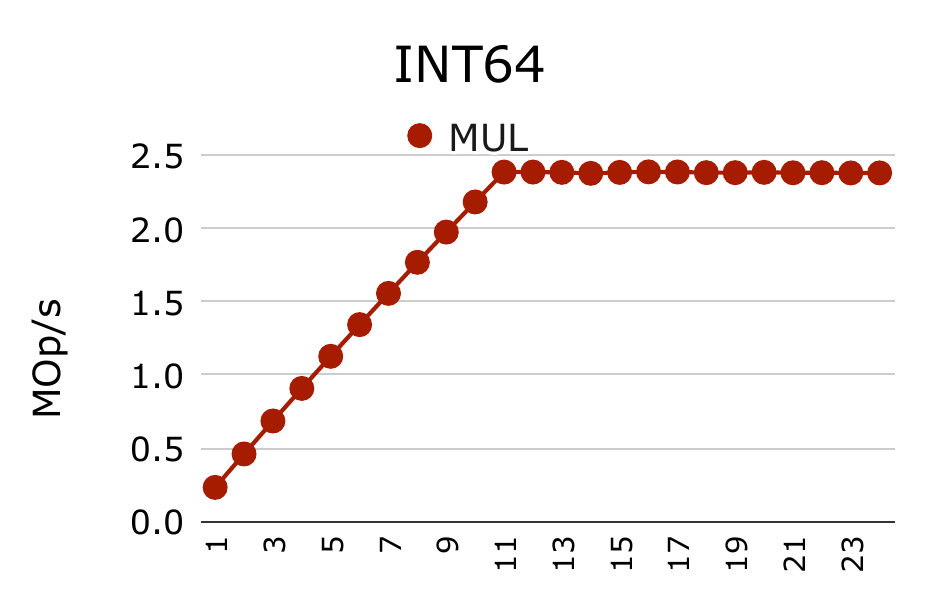}\hspace{4pt}
\includegraphics[width=.3\textwidth]{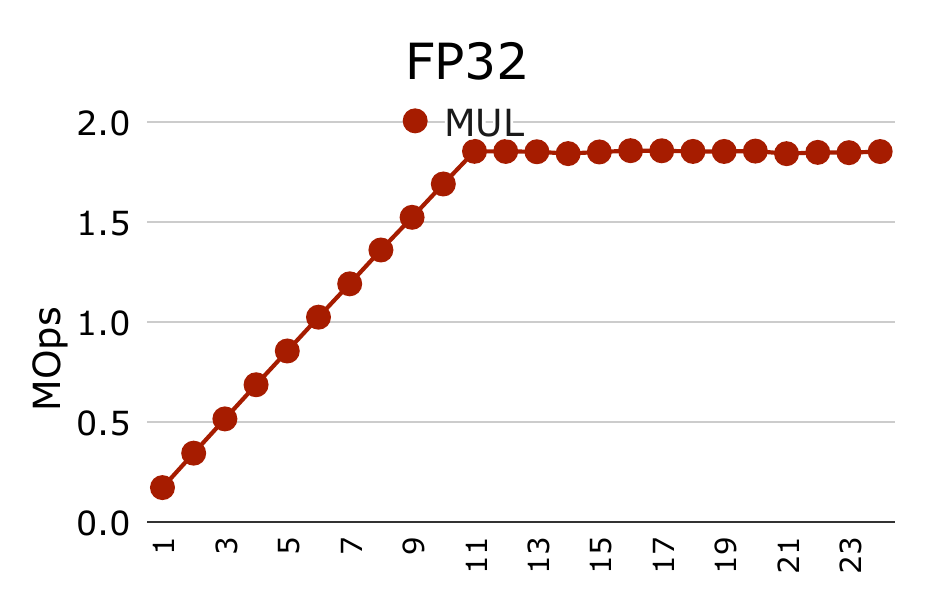}\hspace{4pt}
\includegraphics[width=.3\textwidth]{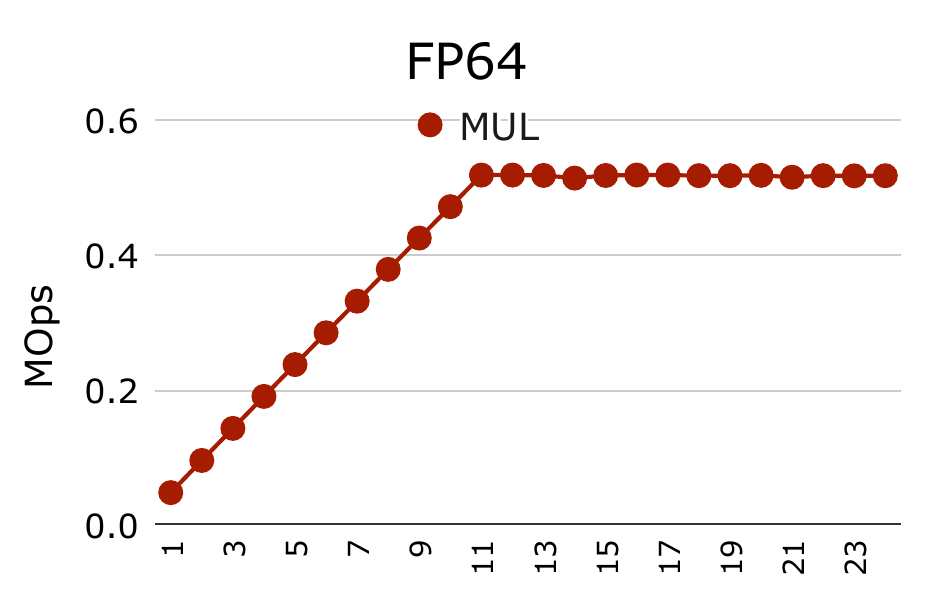}
\end{minipage} % 
\vspace{-12pt}
\caption{Arithmetic throughput achieved on one DPU varying the number of tasklets for all data types.}
\label{fig:1DPU-ai}
\vspace{-8pt}
\end{figure}



\newpage

\section{\SparseP{} Software Package}\label{sec:appendix-sparseP}
Table~\ref{table:appendix-library} summarizes all \spmv{} PIM kernels provides by \SparseP{} library. All kernels support a wide range of data types, i.e., 8-bit integer, 16-bit integer, 32-bit integer, 64-bit integer, 32-bit float, and 64-bit double data types.

\begin{table}[H]
\vspace{-8pt}
\centering
\begin{minipage}{1\linewidth}
%\ra{0.9}
\resizebox{1.0\linewidth}{!}{
\begin{tabular}{| l | l | l | l | l | l |} 
 \toprule
 Partitioning & Compressed & Balancing & Balancing  & Synchronization \\ 
 Technique & Format & Among PIM Cores & Among Threads  & Approach  \\ [0.5ex] \midrule \midrule
% \hline\hline
    \multirow{9}{*}{\hspace*{2.1em}\turnbox{0}{1D}} & \multirow{2}{*}{CSR} &  rows (\textbf{CSR.row}) &  rows, nnz$^{\star}$ & -   \\
    & & nnz$^{\star}$ (\textbf{CSR.nnz}) &  rows, nnz$^{\star}$ & -   \\ \cline{2-5}
    & \multirow{2}{*}{COO} &  rows (\textbf{COO.row}) &  rows, nnz$^{\star}$ & -   \\
    & & nnz$^{\star}$ (\textbf{COO.nnz-rgrn}) &  rows, nnz$^{\star}$ & -   \\
    & & nnz (\textbf{COO.nnz}) &  nnz & lb-cg / lb-fg / lf \\  \cline{2-5}
    & \multirow{2}{*}{BCSR} &  blocks$^{\dagger}$ (\textbf{BCSR.block}) &  blocks, nnz$^{\dagger}$ & lb-cg / lb-fg$^{\dagger}$   \\
    & & nnz$^{\dagger}$ (\textbf{BCSR.nnz}) &  blocks, nnz$^{\dagger}$ & lb-cg / lb-fg$^{\dagger}$ \\  \cline{2-5}
    & \multirow{2}{*}{BCOO} &  blocks (\textbf{BCOO.block}) &  blocks, nnz & lb-cg / lb-fg / lf \\
    & & nnz (\textbf{BCOO.nnz}) &  blocks, nnz & lb-cg / lb-fg / lf  \\ \hline
    \multirow{4}{*}{\shortstack{2D \\ \equallySized}} & CSR (\textbf{dcsr}) & - & rows, nnz$^{\star}$ & -  \\  \cline{2-5}
    &  COO (\textbf{dcoo}) & - & nnz & lb-cg / lb-fg / lf \\  \cline{2-5}
    &  BCSR (\textbf{dbcsr}) & - & blocks, nnz$^{\dagger}$ & lb-cg / lb-fg$^{\dagger}$  \\  \cline{2-5}
    &  BCOO (\textbf{dbcoo}) & - & blocks, nnz & lb-cg / lb-fg  \\ \hline
  \multirow{6}{*}{\shortstack{2D \\ \equallyWidth}} &  CSR (\textbf{rbdcsr}) & nnz$^{\star}$ & rows, nnz$^{\star}$ & -  \\  \cline{2-5}
    &  COO (\textbf{rbdcoo}) & nnz & nnz & lb-cg / lb-fg / lf   \\  \cline{2-5}
    & \multirow{2}{*}{BCSR} & blocks$^{\dagger}$ (\textbf{rbdbcsr}) & blocks, nnz$^{\dagger}$ & lb-cg / lb-fg$^{\dagger}$ \\
    &  & nnz$^{\dagger}$ & blocks, nnz$^{\dagger}$ & lb-cg / lb-fg$^{\dagger}$ \\ \cline{2-5}
    & \multirow{2}{*}{BCOO} & blocks (\textbf{rbdbcoo}) & blocks, nnz & lb-cg / lb-fg   \\ 
    & & nnz  & blocks, nnz & lb-cg / lb-fg   \\ \hline     
  \multirow{6}{*}{\shortstack{2D \\ \variableSized}} &  CSR (\textbf{bdcsr}) & nnz$^{\star}$ & rows, nnz$^{\star}$& -  \\  \cline{2-5}
    &  COO (\textbf{bdcoo}) & nnz  & nnz & lb-cg / lb-fg / lf \\  \cline{2-5}
    &  \multirow{2}{*}{BCSR} & blocks$^{\dagger}$ (\textbf{bdbcsr}) & blocks, nnz$^{\dagger}$ & lb-cg / lb-fg$^{\dagger}$   \\
    &  & nnz$^{\dagger}$ & blocks, nnz$^{\dagger}$ & lb-cg / lb-fg$^{\dagger}$   \\ \cline{2-5}
    &  \multirow{2}{*}{BCOO } & blocks (\textbf{bdbcoo}) & blocks, nnz & lb-cg / lb-fg  \\ 
    &  &  nnz & blocks, nnz &  lb-cg / lb-fg  \\      
 \bottomrule
\end{tabular}
}
\end{minipage} \hspace{2pt}% 
\vspace{-1pt}
\caption{\SparseP{} library. $^{\star}$: row-granularity, $^{\dagger}$: block-row-granularity, $^{\ddagger}$: (only for 8-bit integer and 4x4 block sizes)}
\label{table:appendix-library}
\vspace{-18pt}
\end{table}



\newpage

\section{Large Matrix Dataset}\label{sec:appendix-matrix-dataset}
We present all details for our large matrix data set. Table~\ref{tab:appendix-large-matrices} highlights in red color matrices with a block pattern~\cite{Kourtis2011CSX,Elafrou2018SparseX}, and presents the sparsity of the matrix (i.e., NNZ / (rows x columns)), the standard deviation of non-zero elements among rows (NNZ-r-std) and columns (NNZ-c-std). Table~\ref{tab:appendix-large-matrices-plot} presents a graphic plot for each matrix of our large data set.

% Flops / byte = (2 * nnz) / (8 * nnz + 12 * N), N : matrix dimension
% source: https://github.com/Sable/fait-maison-spmv
% Flops / byte = (2 * nnz) / (sizeof(datatype) * nnz + 12 * N), N : matrix dimension
\begin{table}[H]
\begin{center}
\vspace{-2mm}
\centering
\begin{minipage}{1\linewidth}
%\resizebox{1.0\linewidth}{0.13\textheight}{
%\resizebox{1.0\linewidth}{!}{
\begin{tabular}{|l|c|r|r|r|r|}
    \toprule
    \textbf{Matrix Name} & \textbf{Rows x Columns} & \textbf{NNZs} & \textbf{Sparsity} & \textbf{NNZ-r-std} & \textbf{NNZ-c-std} \\
    \midrule
    hugetric-00020 & 7122792 x 7122792 & 21361554 & 4.21e-07 & 0.031 & 0.031 \\ \hline 
    
    mc2depi & 525825 x 525825	 & 2100225 & 7.59e-06 & 0.076 & 0.076 \\ \hline 
    
    parabolic\_fem &	525825	 x 525825 & 	3674625 & 	1.33e-05 & 0.153 &  0.153 \\ \hline 
    
    roadNet-TX & 	1393383	x 1393383	& 3843320 & 	1.98e-06 &  1.037 & 1.037 \\ \hline 
    
    rajat31 & 	4690002	 x 4690002 & 	20316253 &  9.24e-07  & 1.106  & 1.106 \\ \hline 
    
    \textcolor{darkred}{af\_shell1} & 	504855 x 	504855	& 17588875 & 	6.90e-05 & 1.275 & 1.275 \\ \hline  
    
    delaunay\_n19 & 	524288 x 	524288 &	3145646 & 	1.14e-05 &  1.338 & 1.338 \\ \hline 
    
    thermomech\_dK  &	204316 x 	204316 & 	2846228 & 6.81e-05 & 1.431 &  1.431 \\ \hline
    
    memchip & 2707524 x 2707524	& 14810202 & 	2.02e-06 &  2.062 & 1.173 \\ \hline 
        
    amazon0601 & 403394 x 403394	& 3387388 & 	2.08e-05 &  2.79 & 15.29  \\ \hline 
    
    FEM\_3D\_thermal2 & 147900 x 	147900 & 	3489300 & 	1.59e-04 & 4.481  & 4.481 \\ \hline 

    %\bottomrule
%\end{tabular}
%}
%\end{minipage} \hspace{2pt}% 
%\begin{minipage}{.49\linewidth}
%\resizebox{1.0\linewidth}{!}{
%\begin{tabular}{|l|c|r|r|r|r|}
%    \toprule
%    \textbf{Matrix Name} & \textbf{Rows x Columns} & \textbf{NNZs} & \textbf{Sparsity} & \textbf{NNZ-r-std} & \textbf{NNZ-c-std} \\
    %\midrule
     
    web-Google	& 916428 x 	916428 & 	5105039 & 	6.08e-06 & 6.557 &  38.366 \\ \hline
    
    \textcolor{darkred}{ldoor}	 & 952203 x 952203	& 46522475 & 	5.13e-05  & 11.951 & 11.951 \\ \hline 
    
    poisson3Db & 	85623 x 85623	 & 2374949 & 	3.24e-04  & 14.712  & 14.712 \\ \hline 
    
    \textcolor{darkred}{boneS10} & 	914898  x 	914898 & 	55468422 & 	6.63e-05 &  20.374 &  20.374 \\ \hline 
    
    webbase-1M	& 1000005 x 1000005	& 3105536 & 	3.106e-06 & 25.345  & 36.890 \\ \hline  
    
    in-2004 & 1382908  x 	1382908	 & 16917053 & 	8.846e-06  & 37.230 & 144.062 \\ \hline 
    
    \textcolor{darkred}{pkustk14} & 	151926  x	151926	 & 14836504 & 	6.428e-04 &  46.508  & 46.508 \\ \hline  
    
    com-Youtube & 	1134890	 x  1134890	 & 5975248 & 4.639e-06  & 50.754  & 50.754 \\ \hline 

    
    sx-stackoverflow &	2601977	 x  2601977 & 	36233450 & 	5.352e-06 &  137.849 & 65.367 \\ \hline 
    
    as-Skitter & 	1696415 x	1696415	& 22190596 & 	7.71e-06  & 136.861 &  136.861 \\ \hline 
    
    ASIC\_680 & 	682862 x  682862 & 	3871773 & 	8.303e-06  & 659.807 & 659.807 \\ \hline 
 
    \bottomrule
\end{tabular}
%}
\end{minipage}%
\end{center}
\caption{Matrix Dataset. Matrices are sorted on their irregular pattern (NNZ-r-std, NNZ-c-std metrics).}
\label{tab:appendix-large-matrices}
\vspace{-8pt}
\end{table}



\newpage

\begin{table}[H]
\begin{center}
\vspace{-2mm}
\centering
\begin{minipage}{0.5\linewidth}
%\resizebox{1.0\linewidth}{0.13\textheight}{
%\resizebox{1.0\linewidth}{!}{
\centering
\begin{tabular}{|l|c|}
    \toprule
    \textbf{Matrix Name} & \textbf{Plot} \\
    \midrule
    hugetric-00020 & \includegraphics[width=0.23\textwidth]{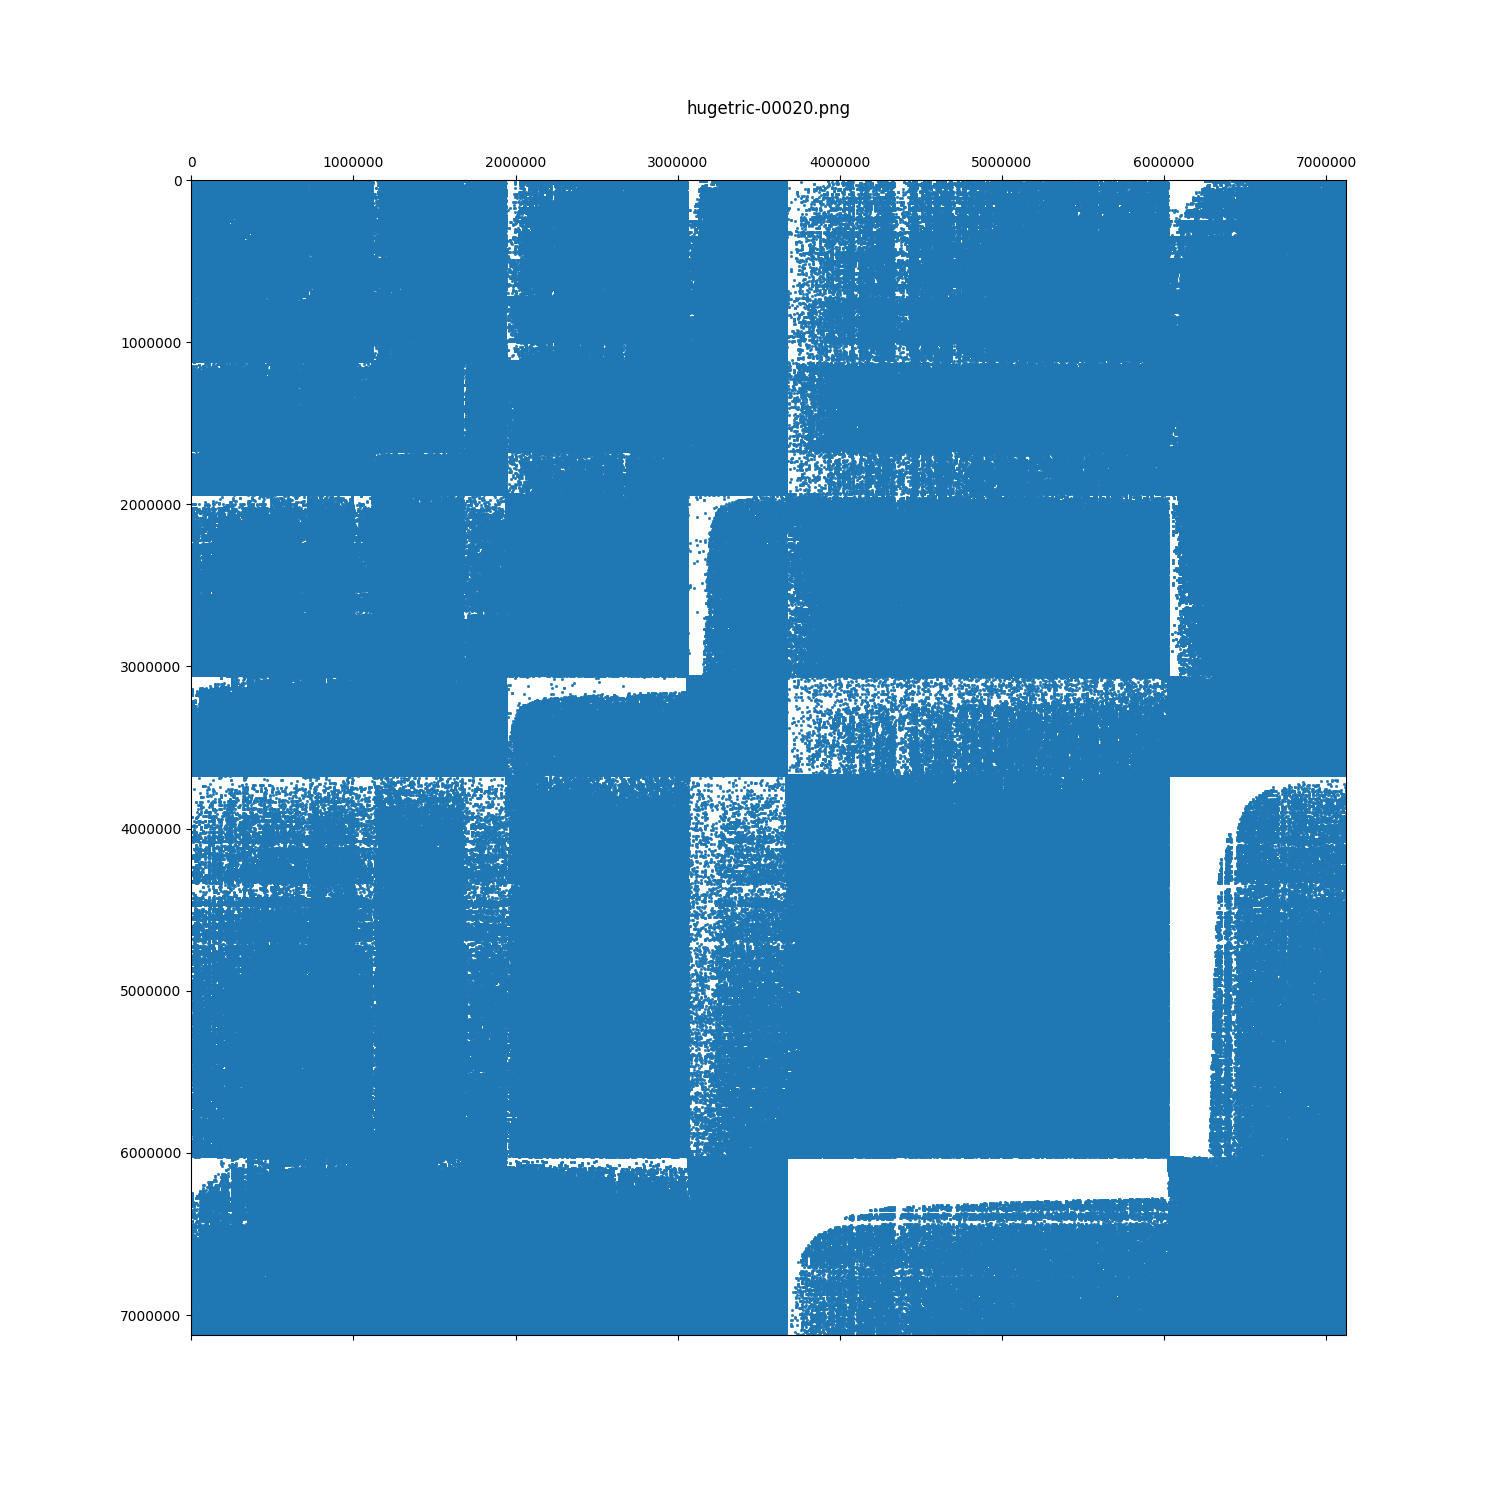} \\ \hline 
    
    mc2depi & \includegraphics[width=0.23\textwidth]{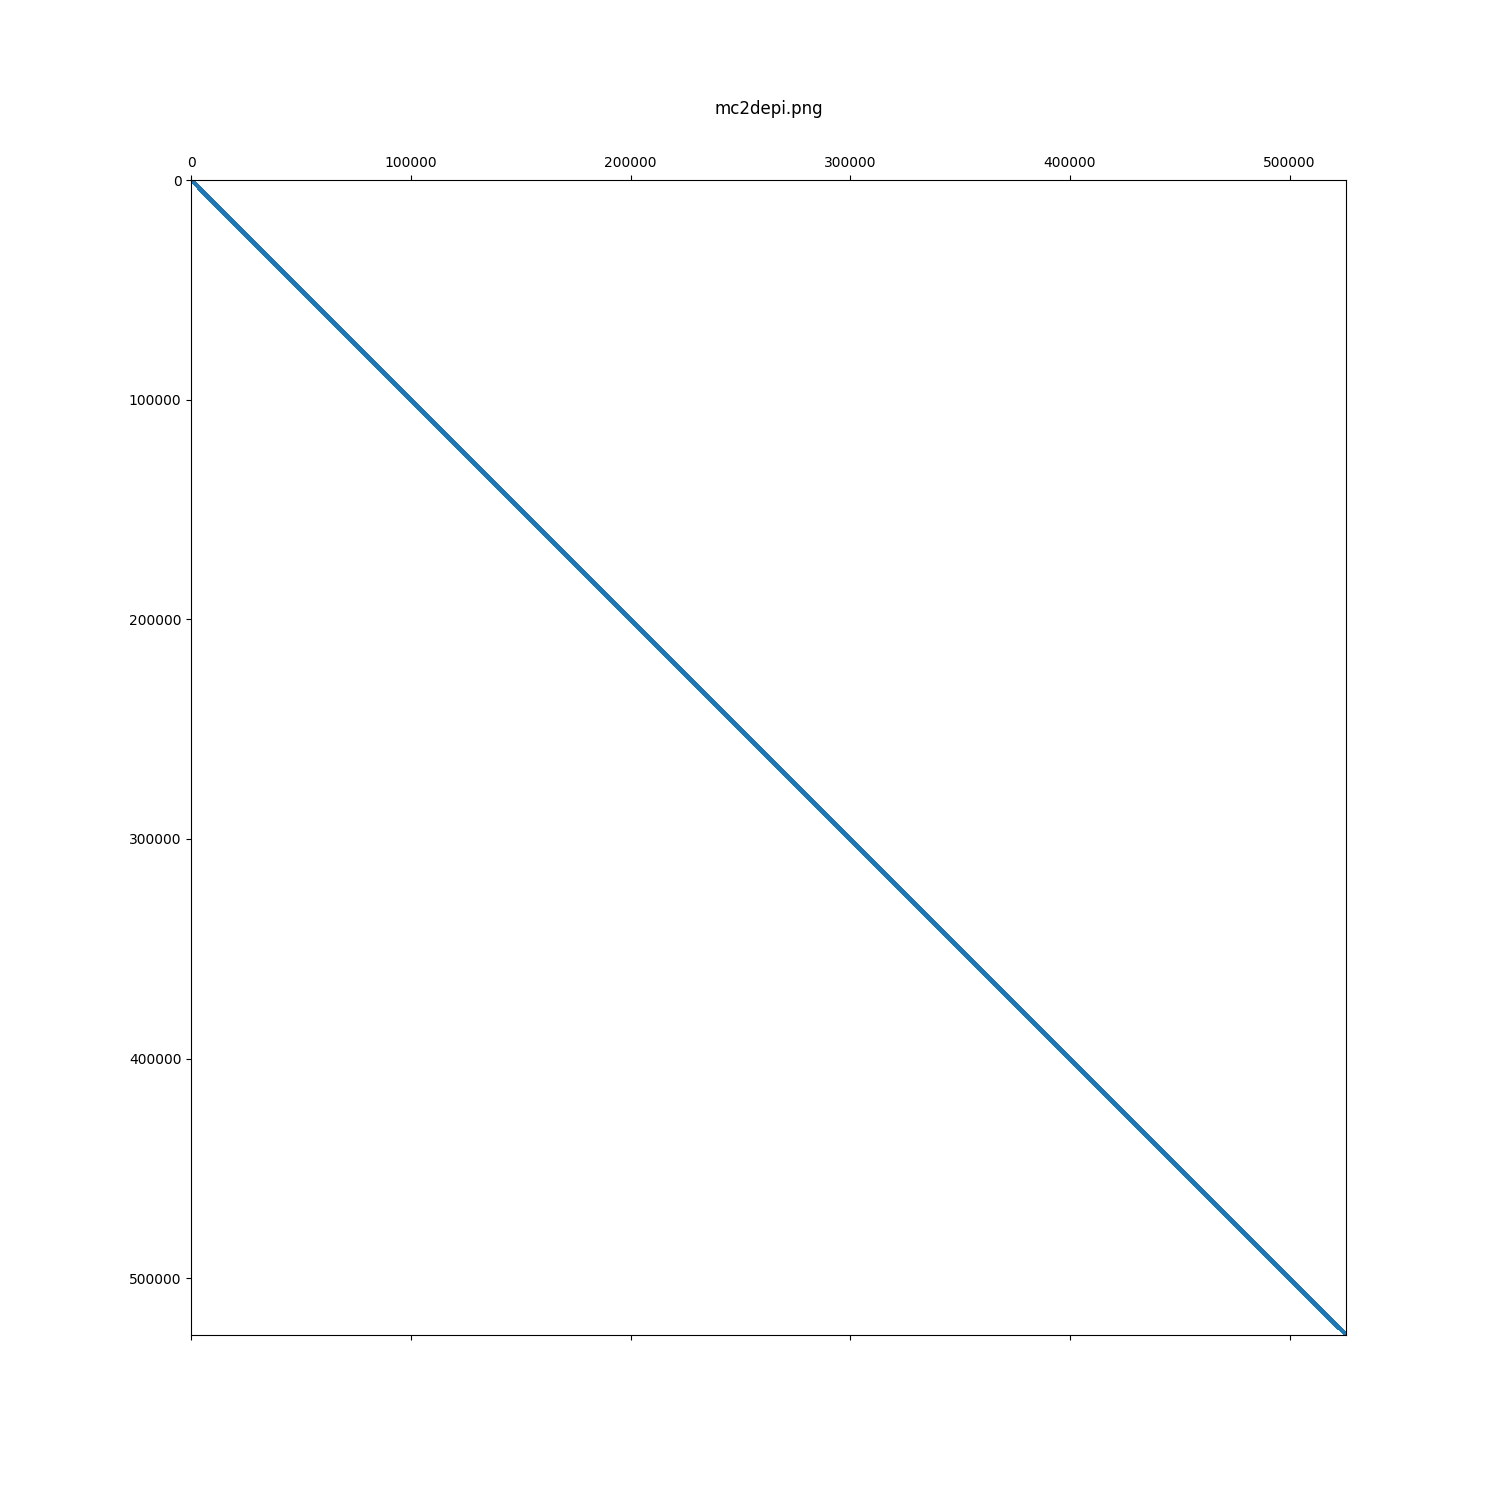} \\ \hline 
    
    parabolic\_fem & \includegraphics[width=0.23\textwidth]{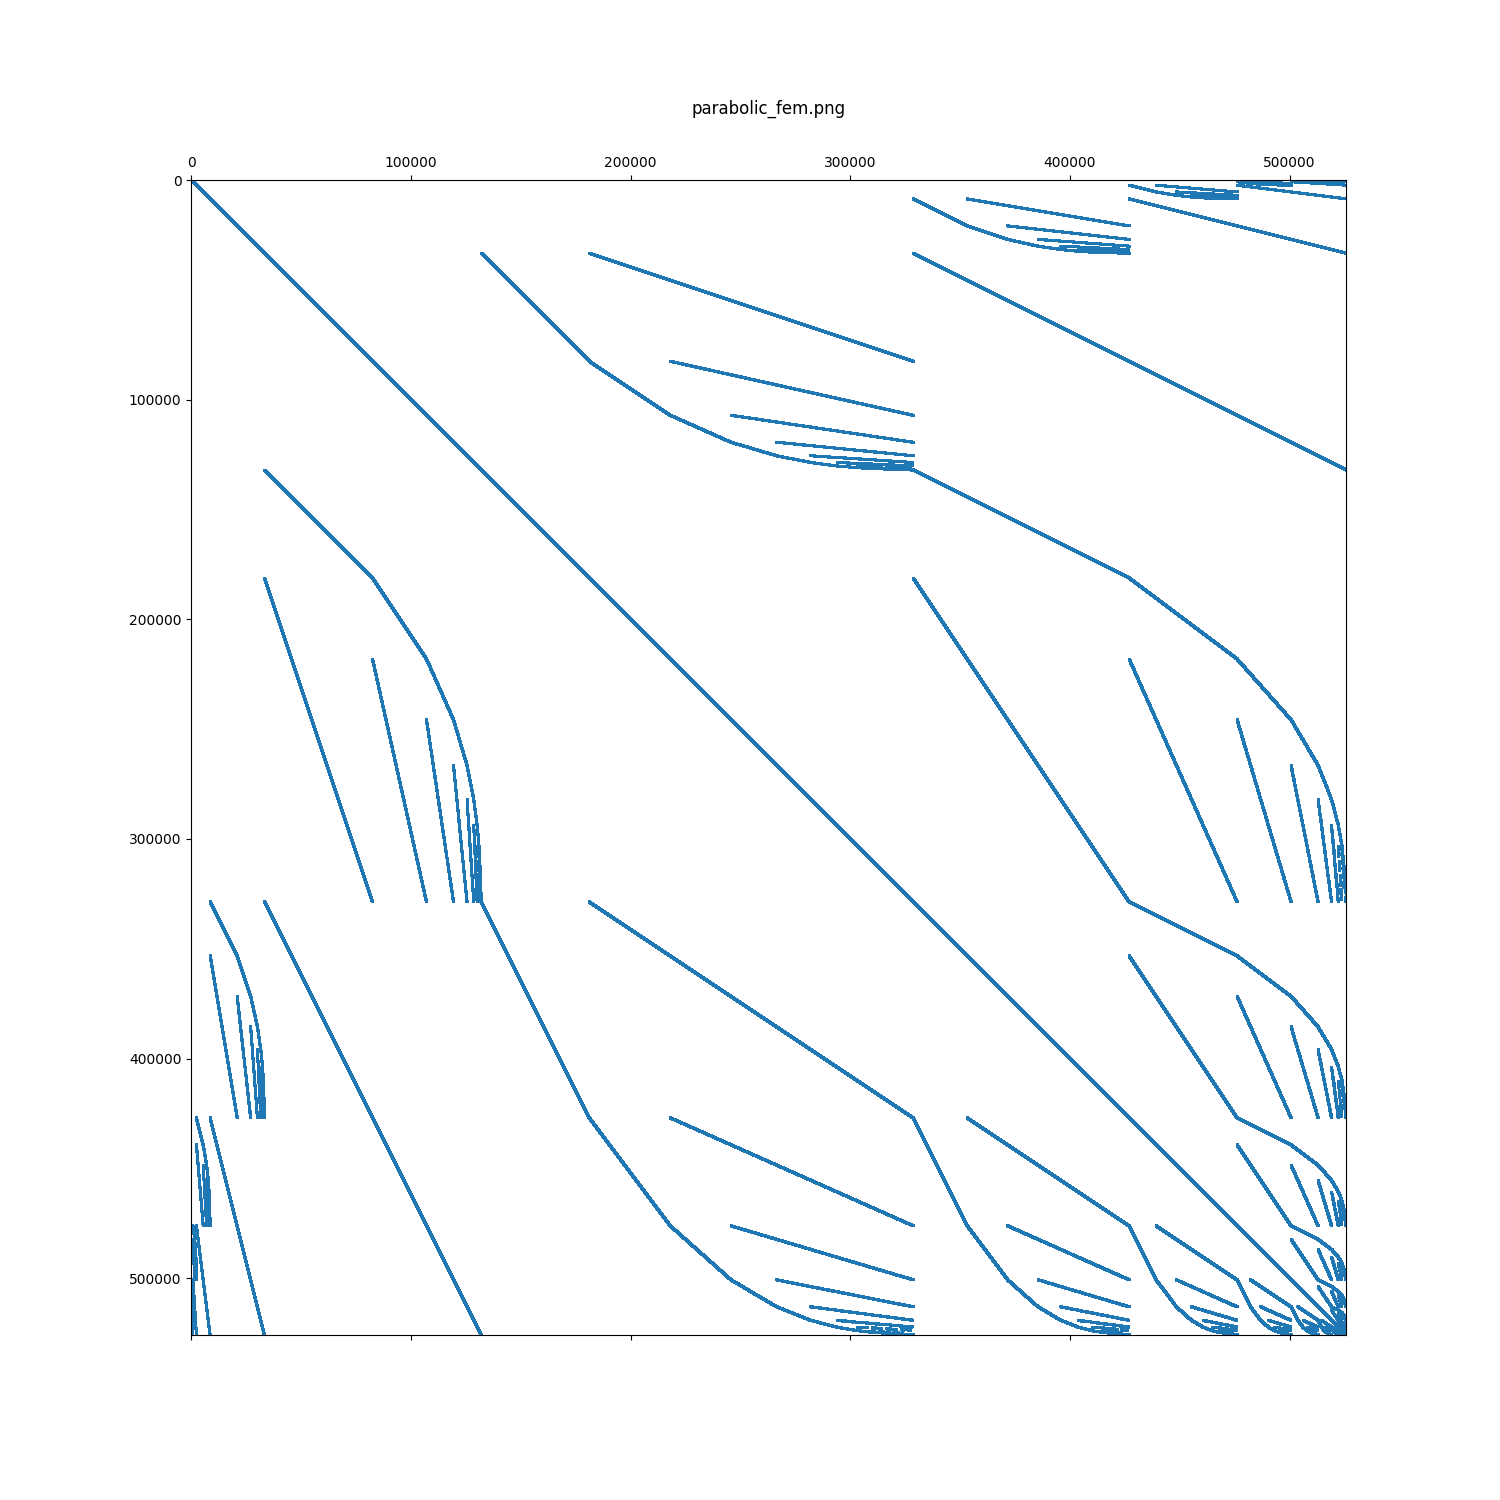} \\ \hline 
    
    roadNet-TX &  \includegraphics[width=0.23\textwidth]{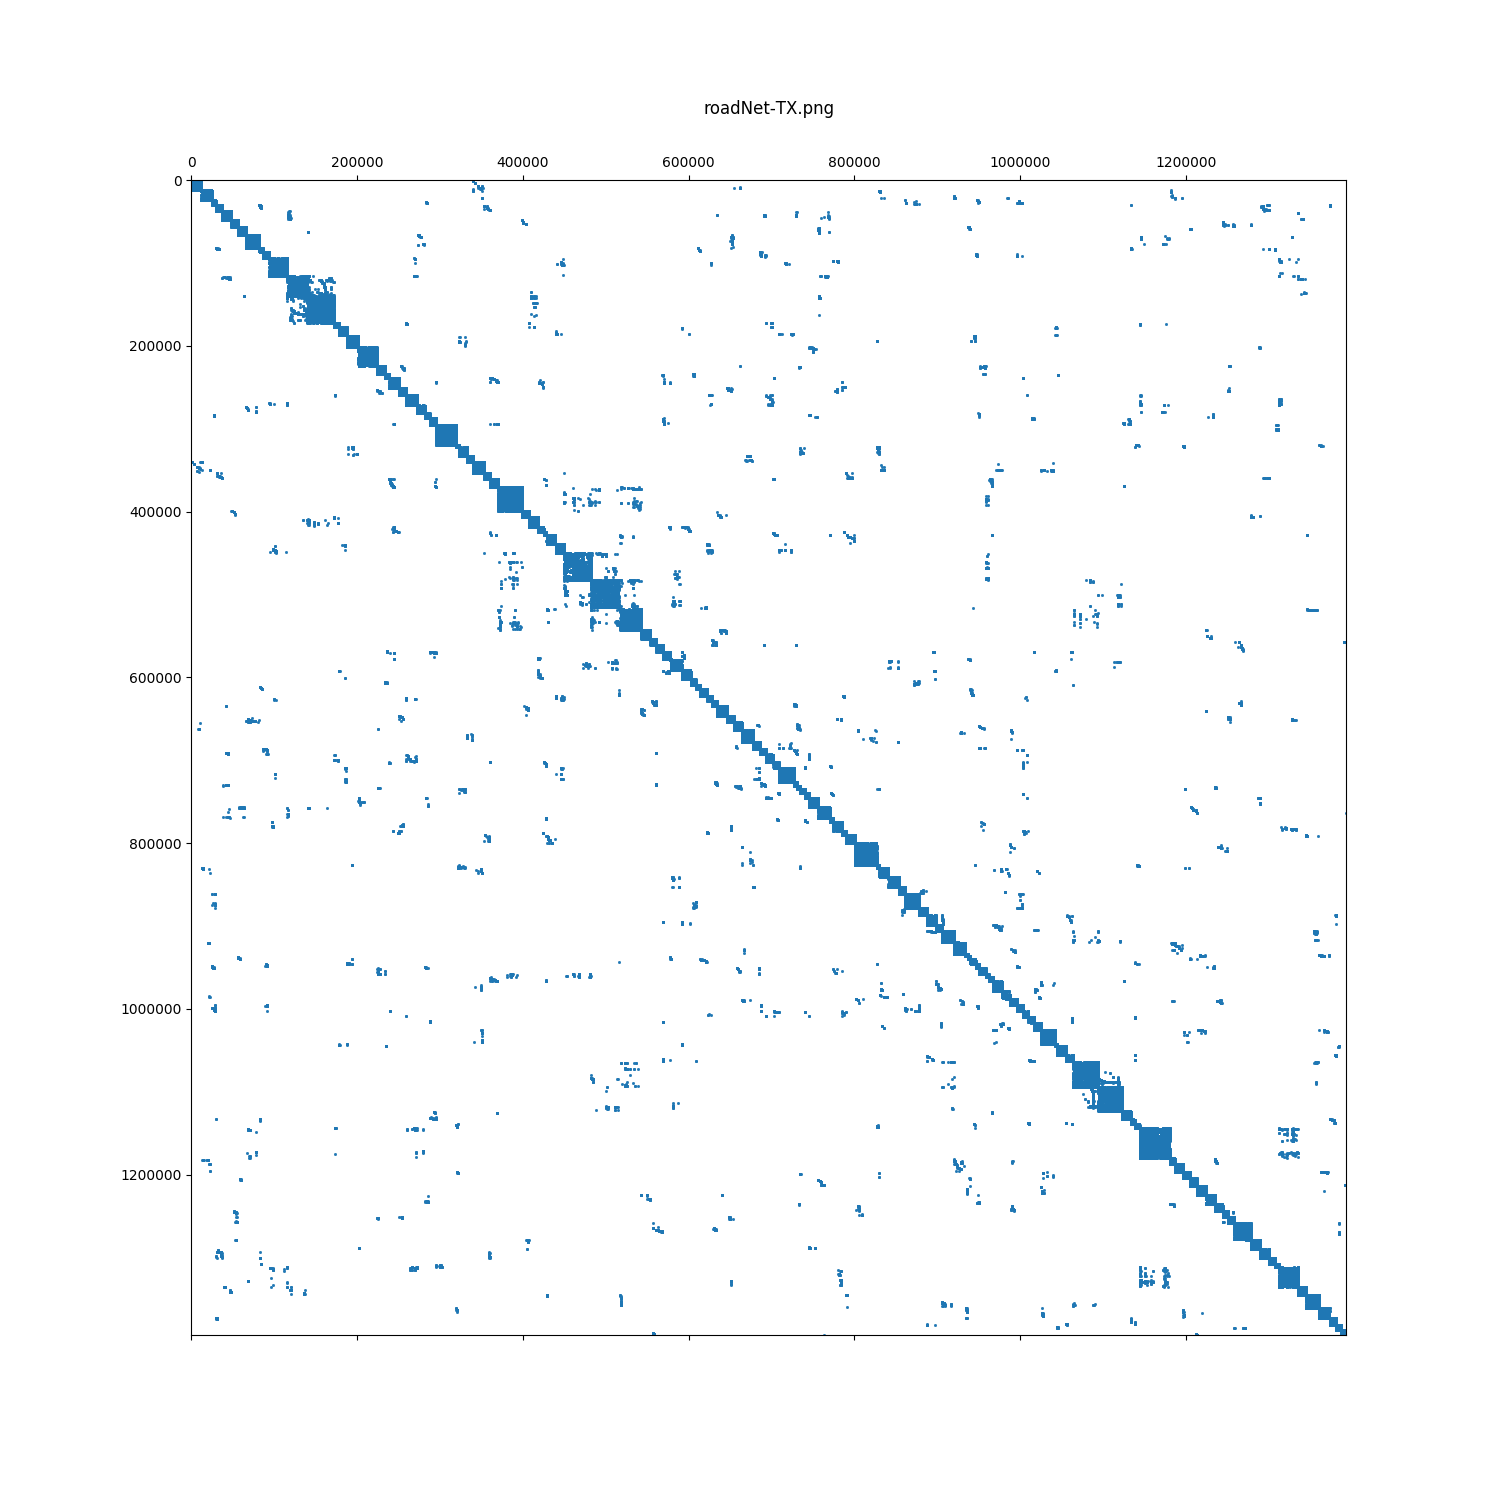} \\ \hline 
    
    rajat31 & 	\includegraphics[width=0.23\textwidth]{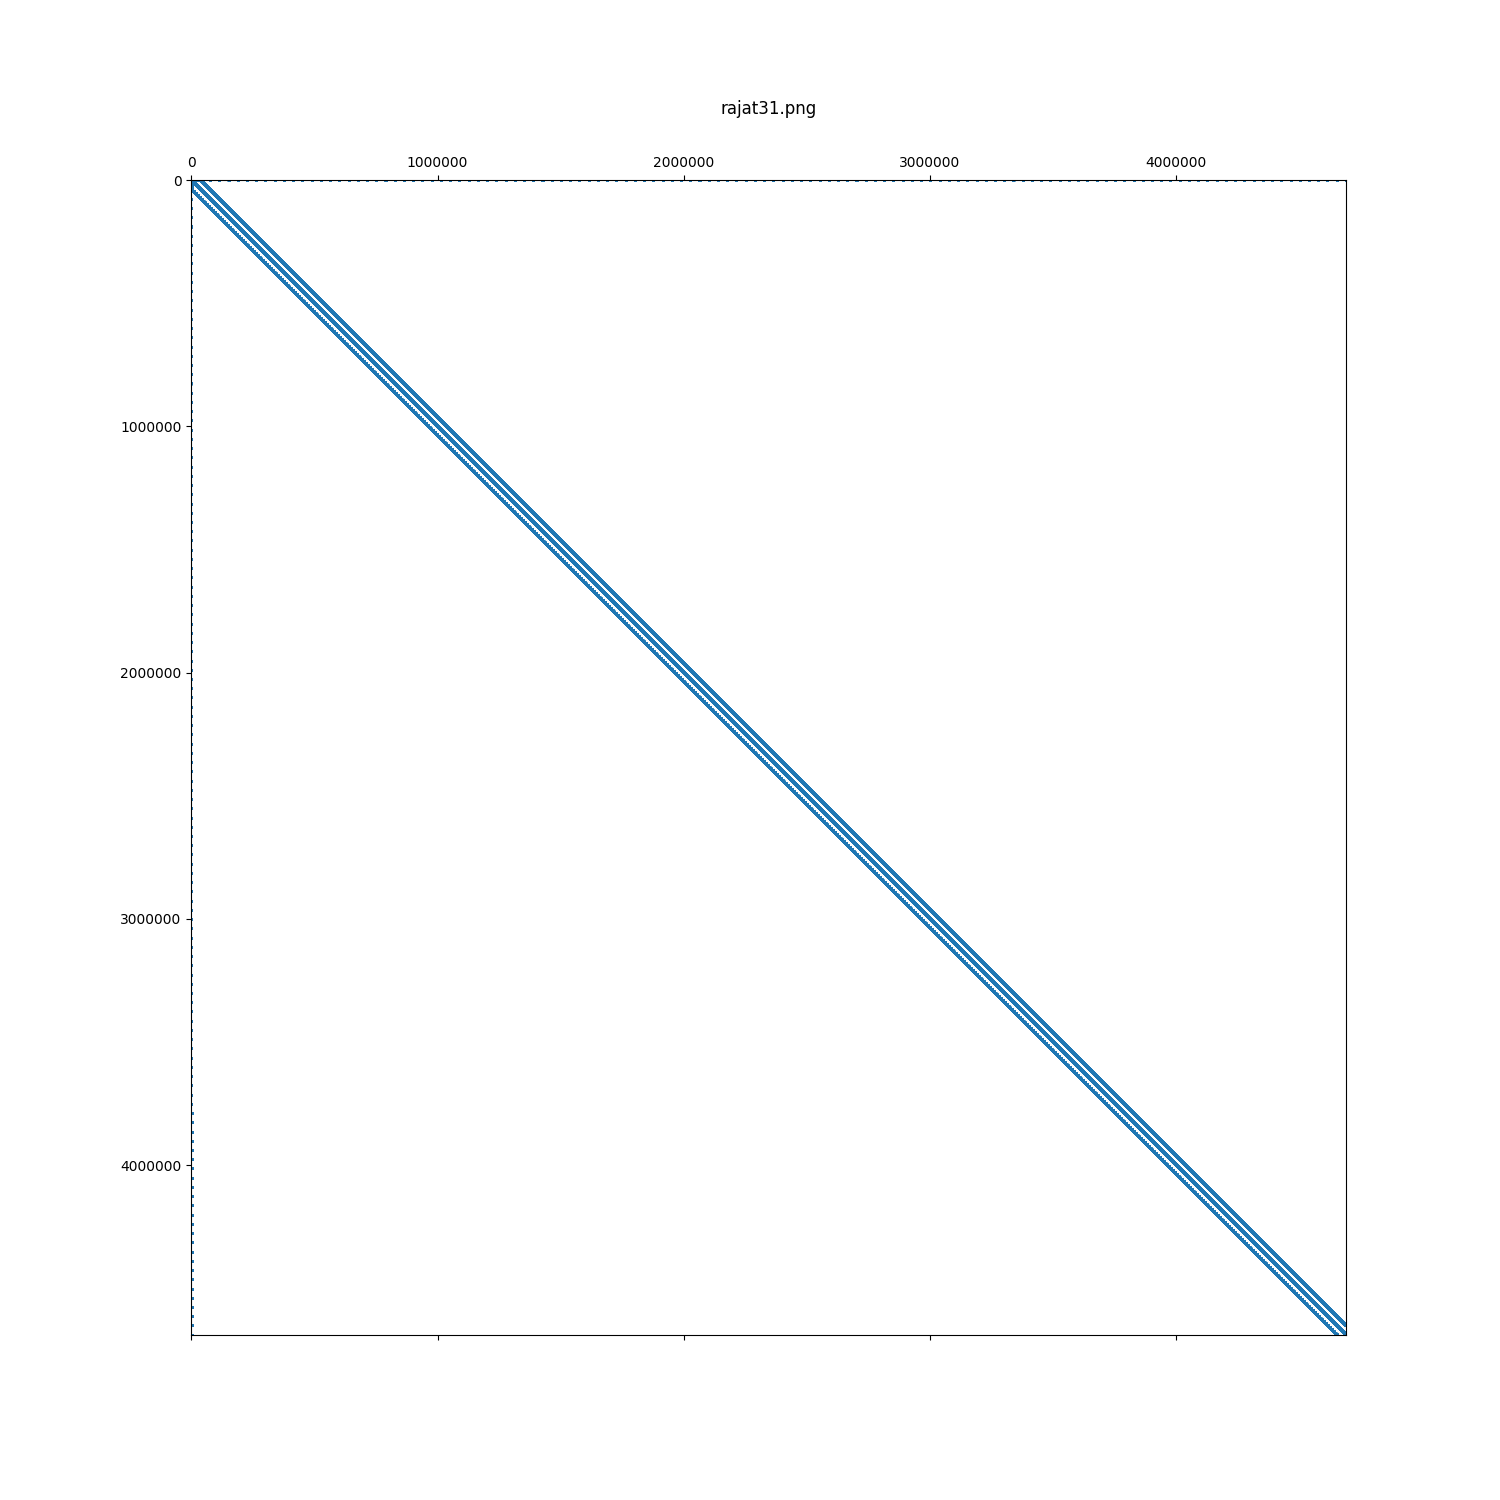} \\ \hline 
    
    \textcolor{darkred}{af\_shell1} & 	\includegraphics[width=0.23\textwidth]{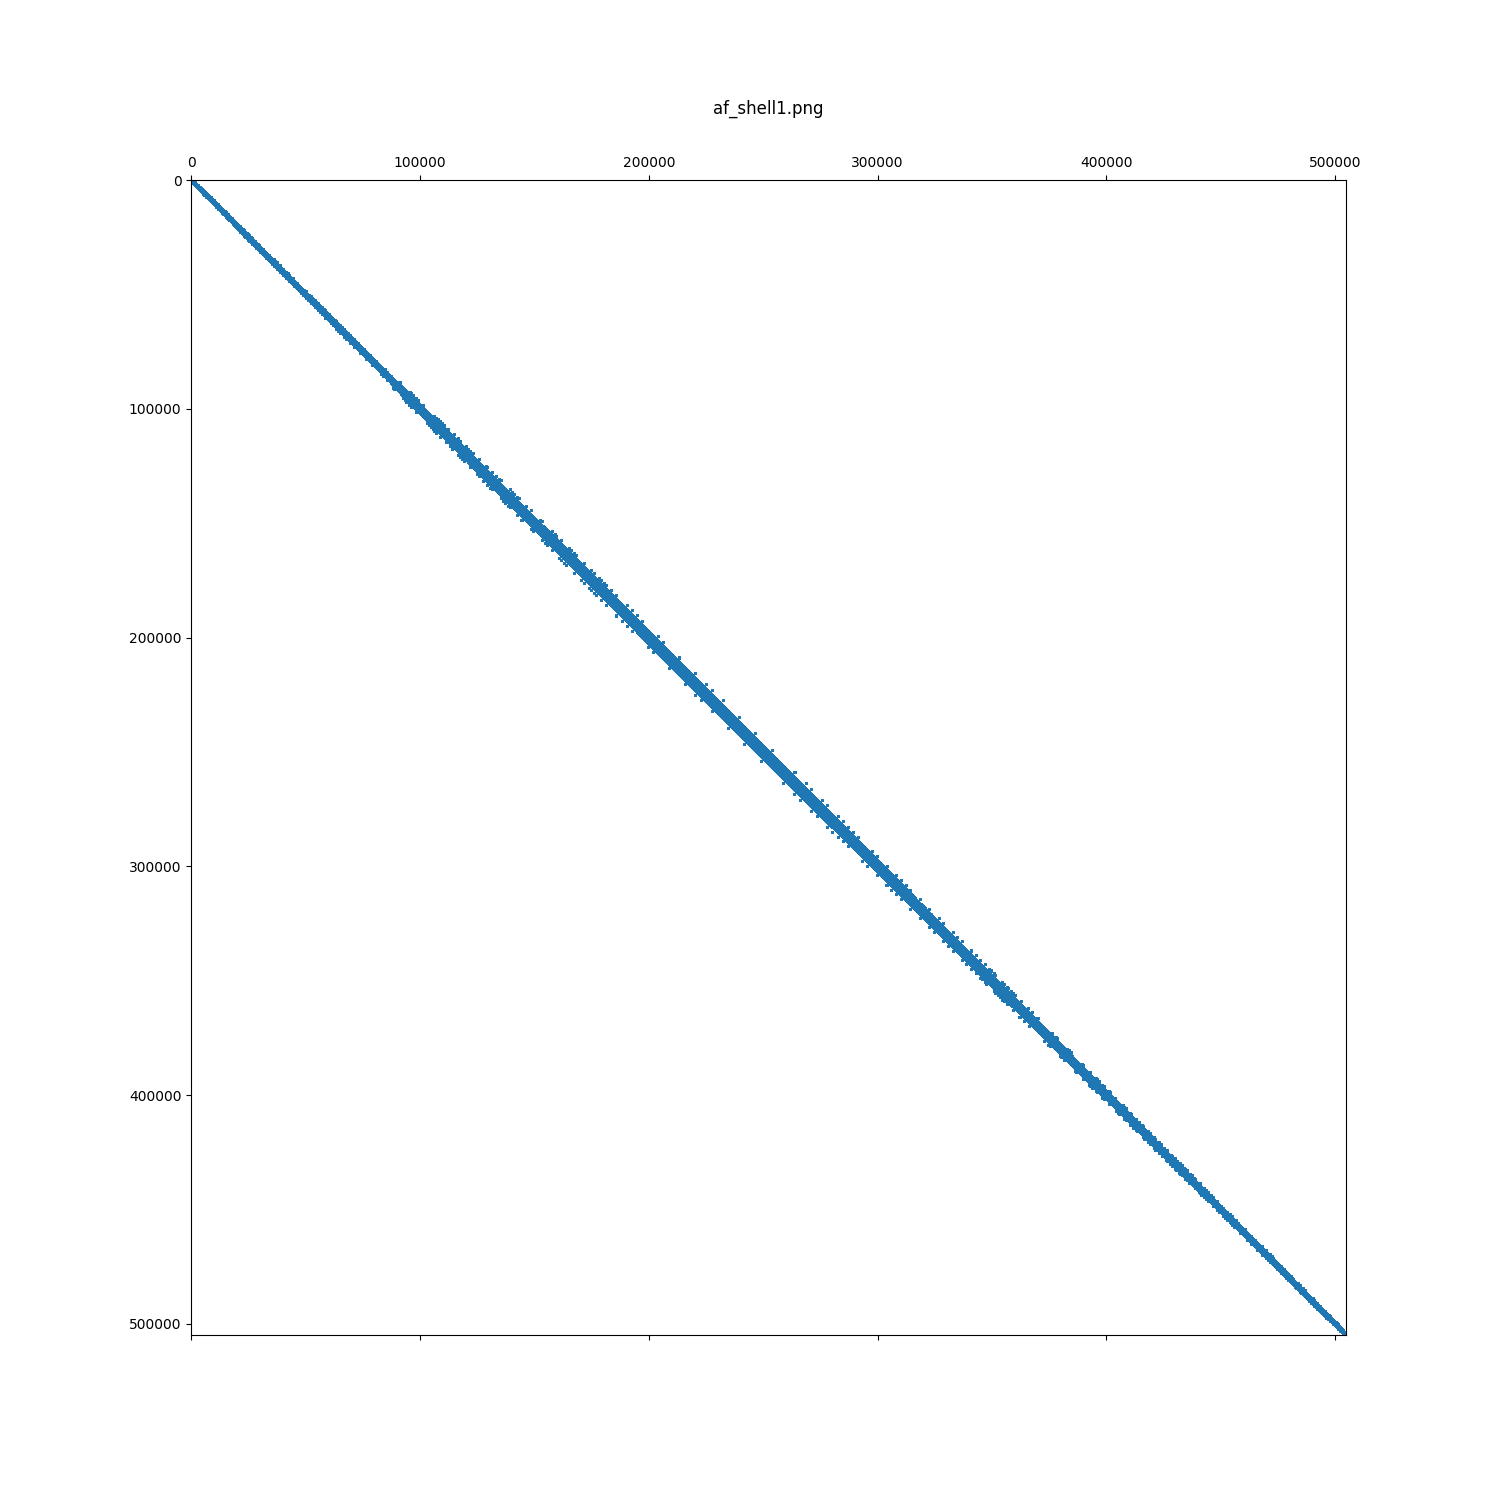} \\ \hline  
    
    delaunay\_n19 & \includegraphics[width=0.23\textwidth]{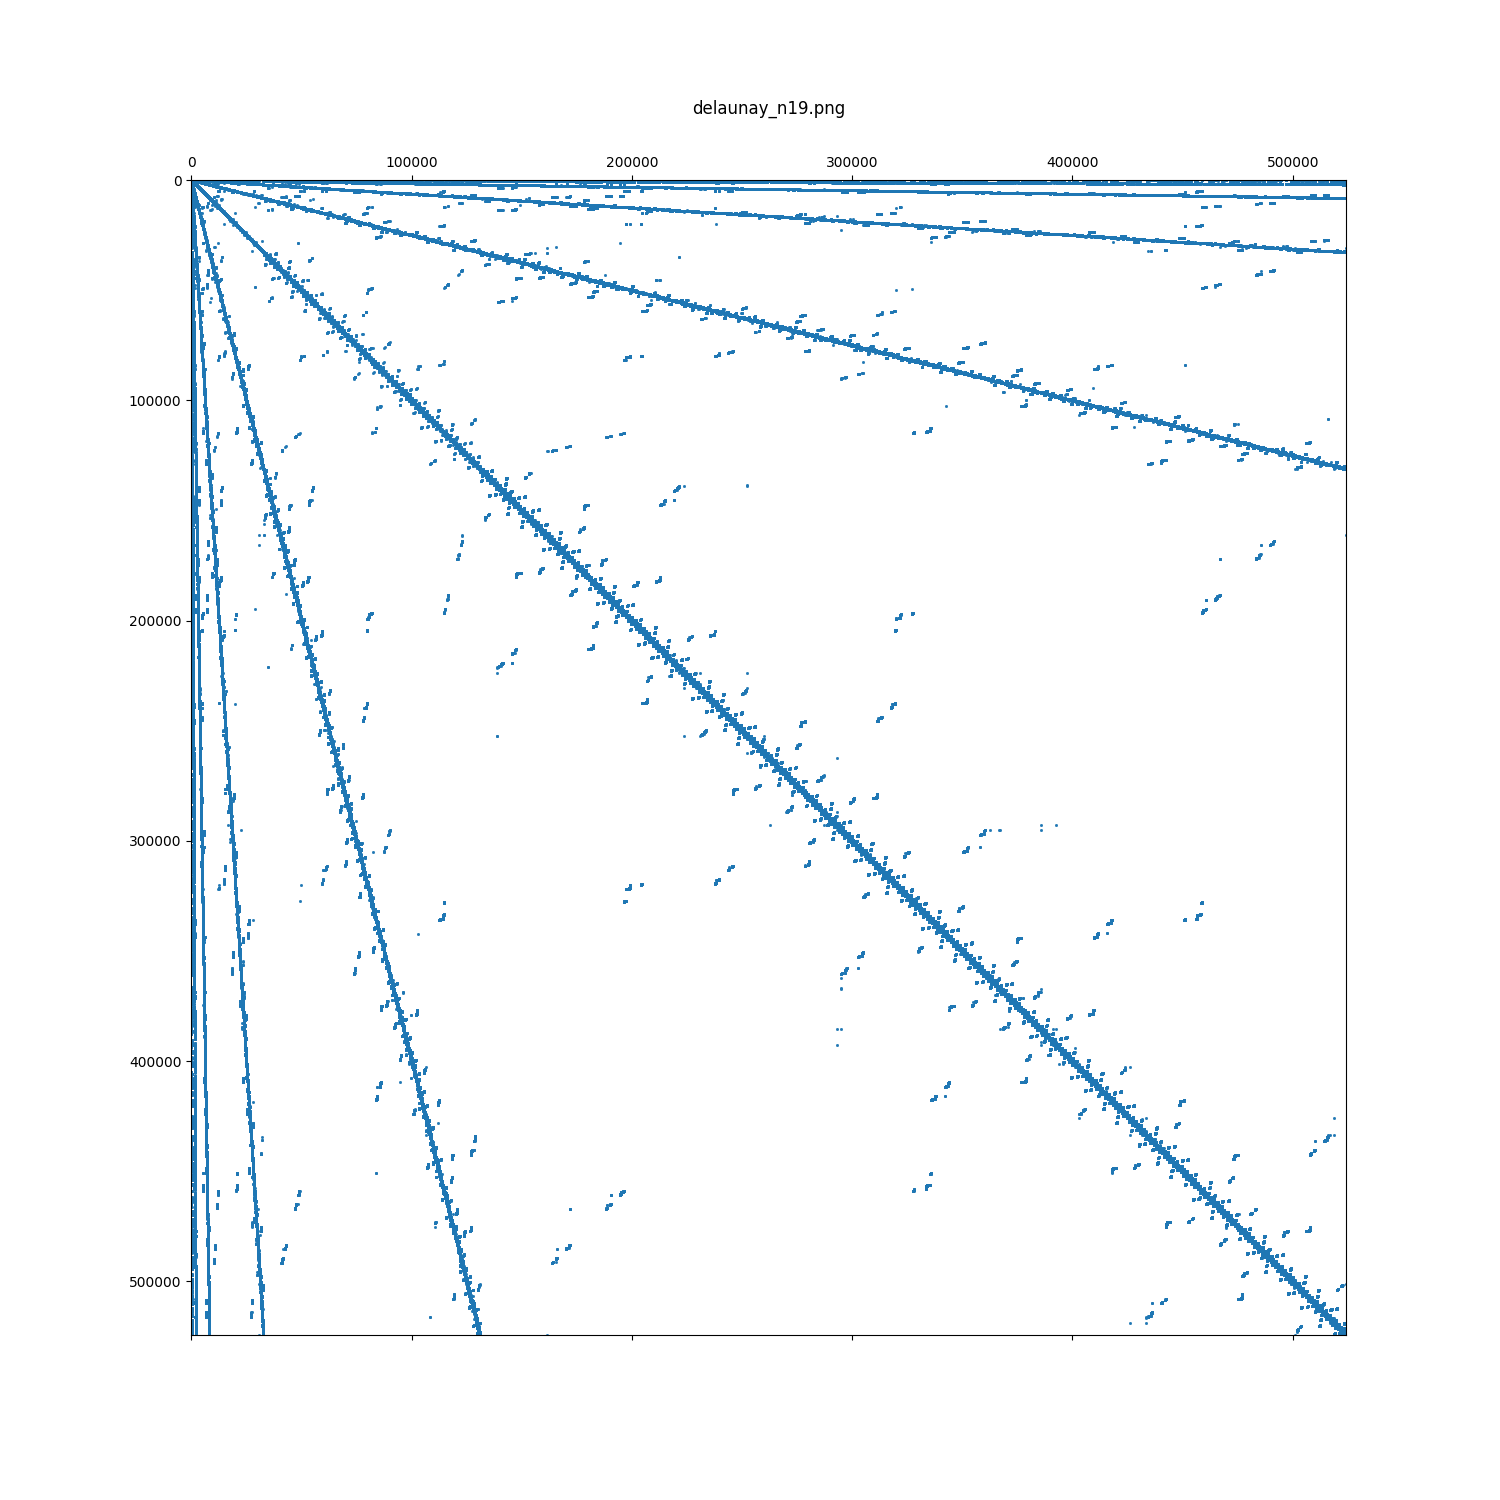}  \\ \hline 
    
    thermomech\_dK  & \includegraphics[width=0.23\textwidth]{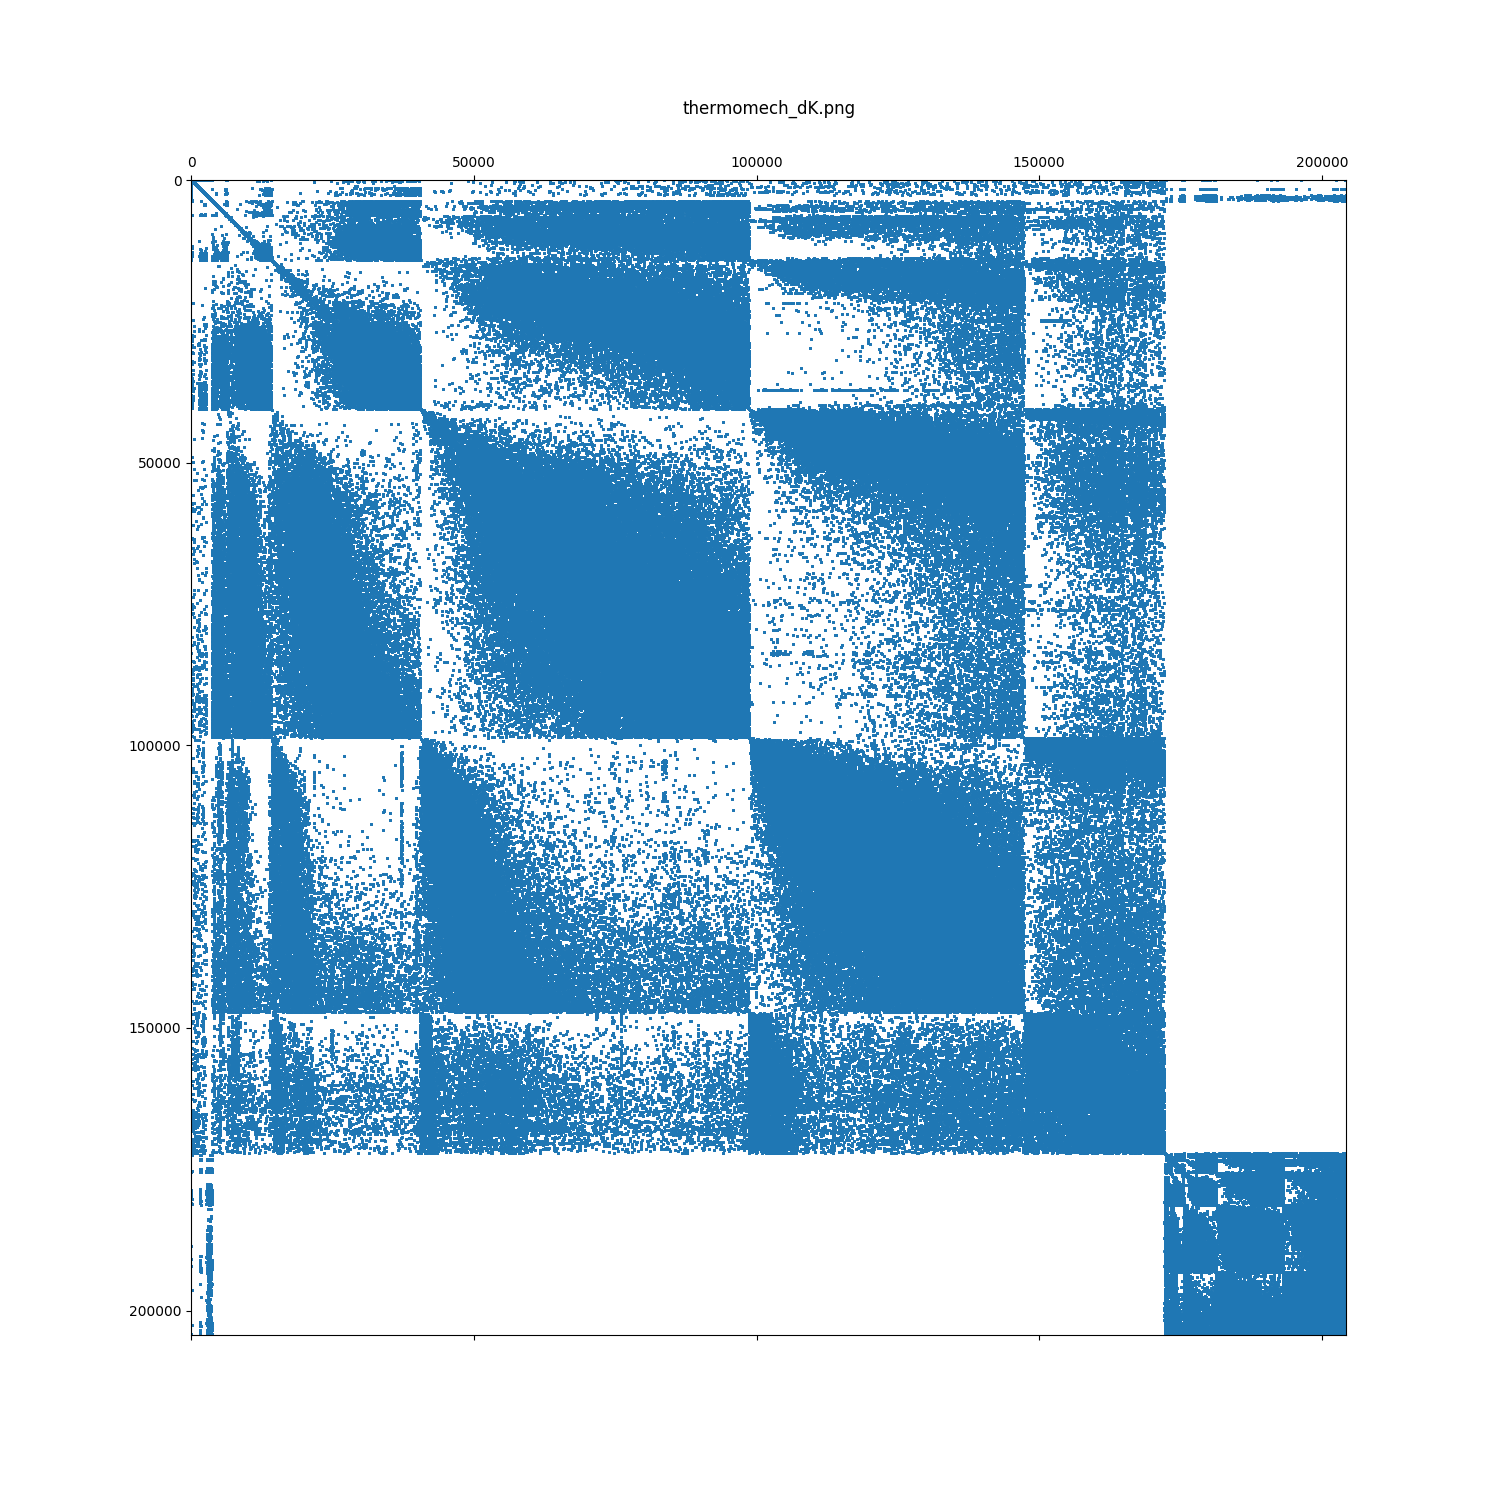} \\ \hline
    
    memchip &  \includegraphics[width=0.23\textwidth]{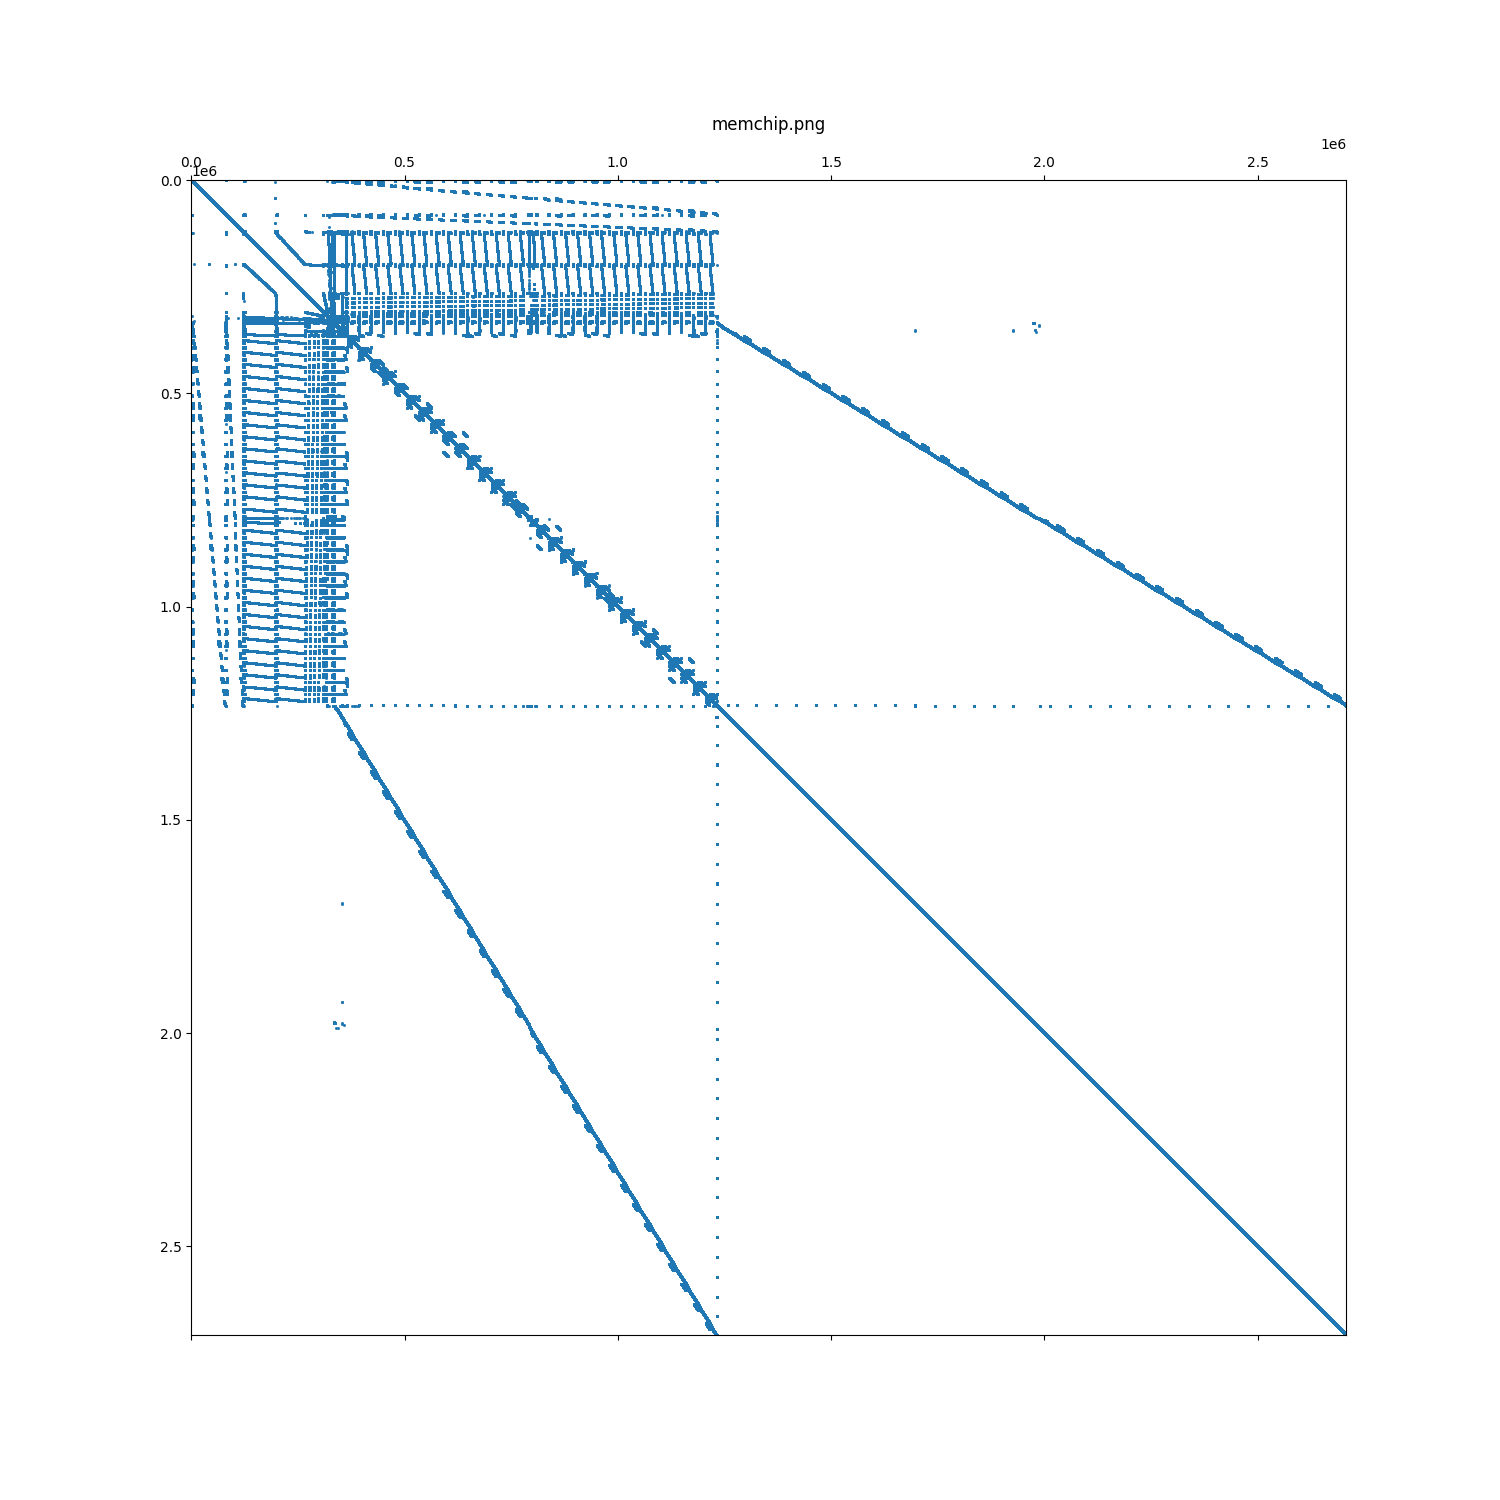} \\ \hline 
        
    amazon0601 & \includegraphics[width=0.23\textwidth]{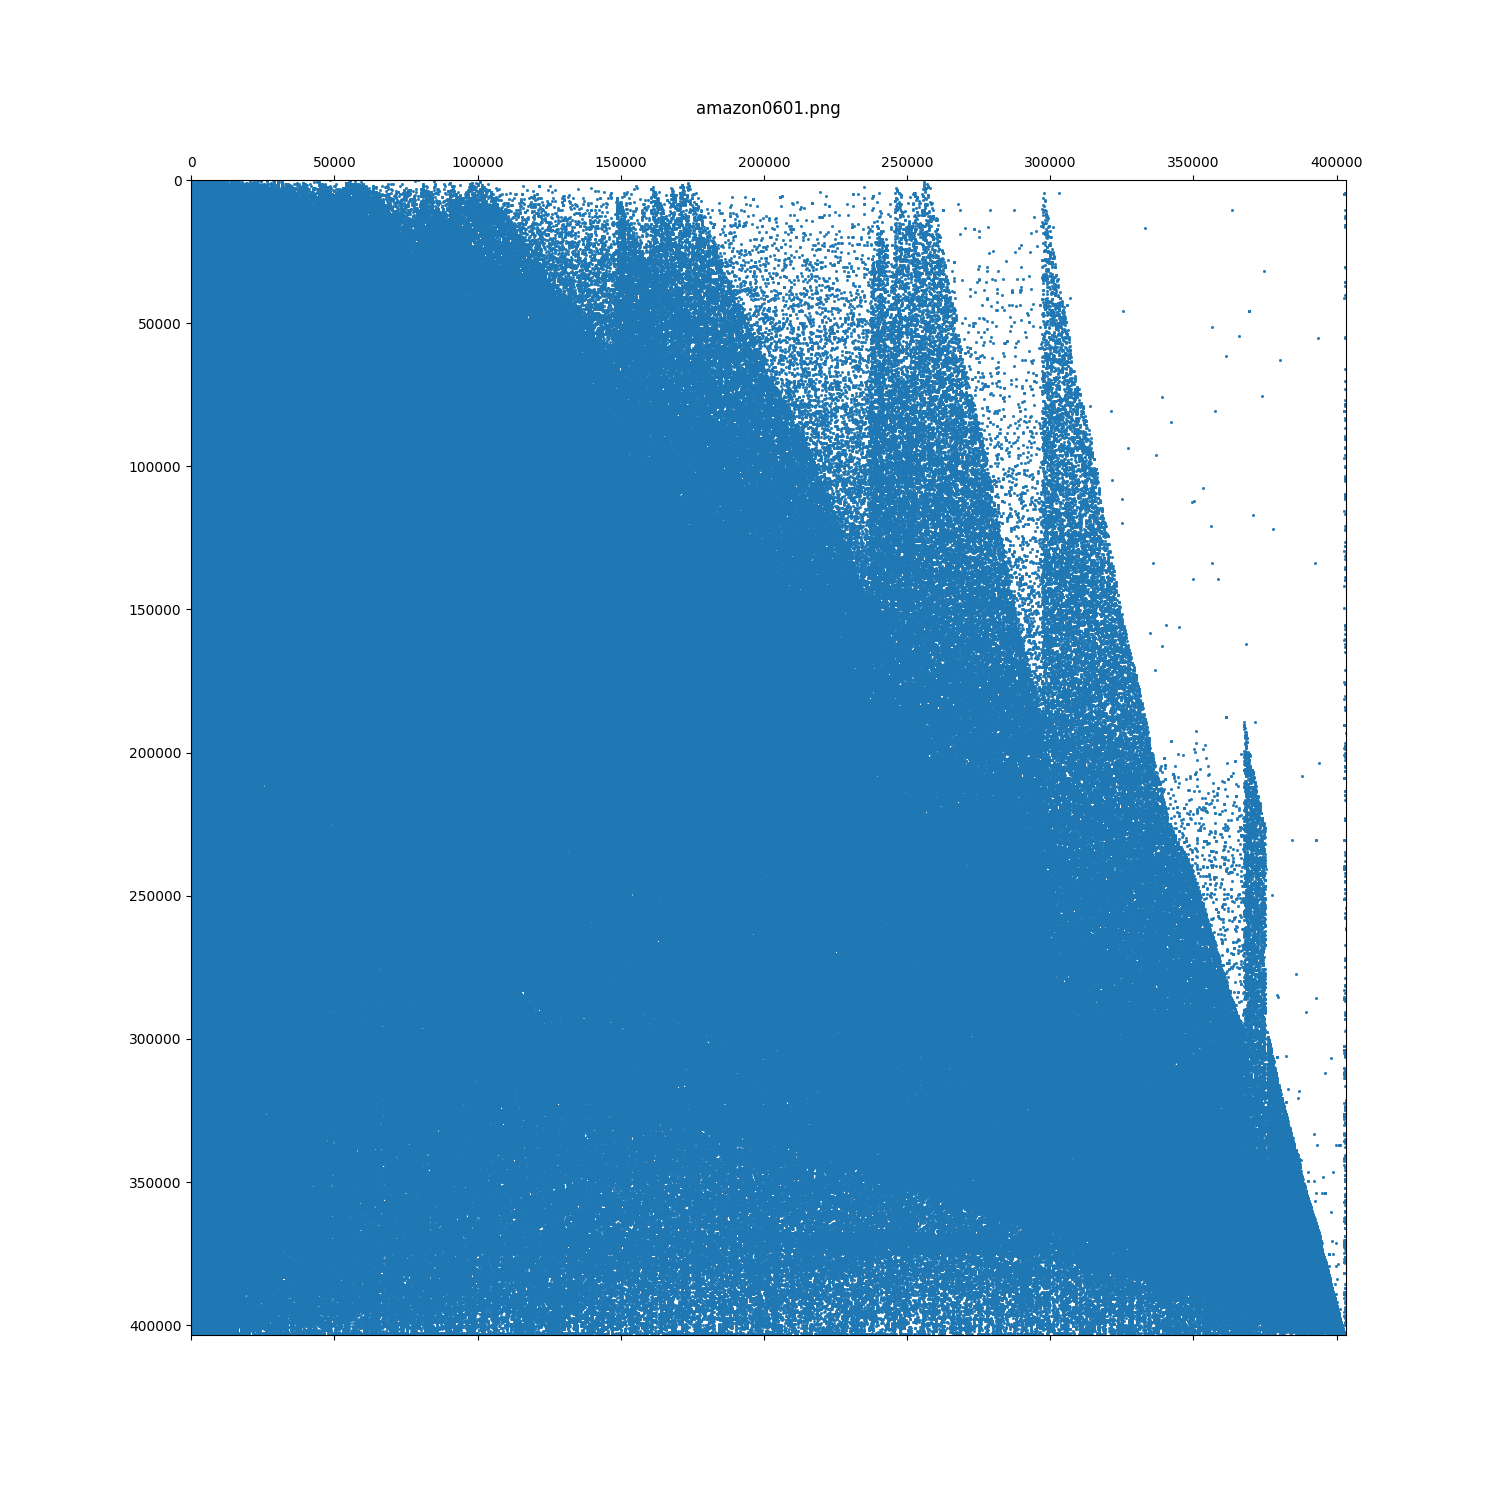} \\ \hline 
    
    FEM\_3D\_thermal2 & \includegraphics[width=0.23\textwidth]{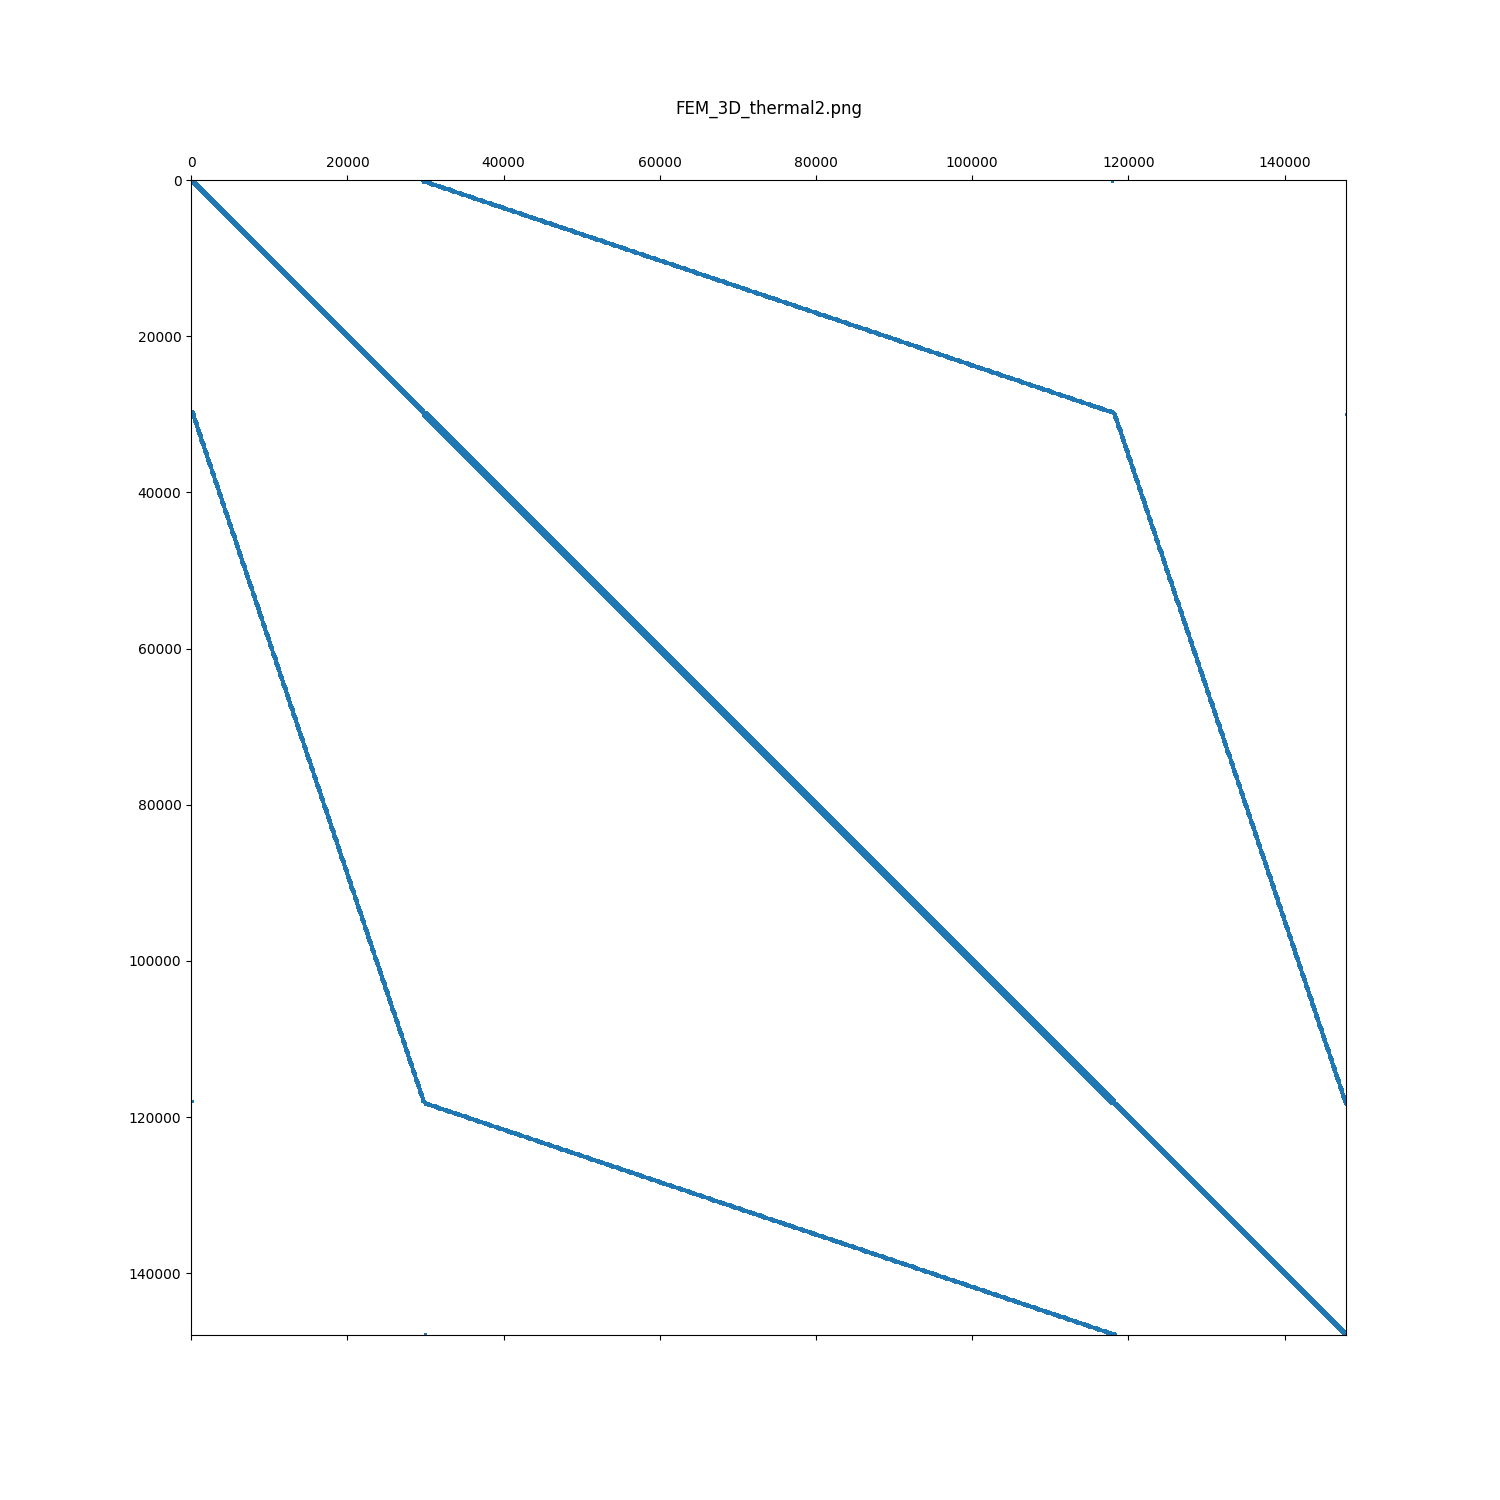}\\ \hline
    \bottomrule
\end{tabular}
%}
\end{minipage}%
\begin{minipage}{0.5\linewidth}
%\resizebox{1.0\linewidth}{0.13\textheight}{
%\resizebox{1.0\linewidth}{!}{
\centering
\begin{tabular}{|l|c|}
    \toprule
    \textbf{Matrix Name} & \textbf{Plot} \\
    \midrule
    web-Google	& \includegraphics[width=0.23\textwidth]{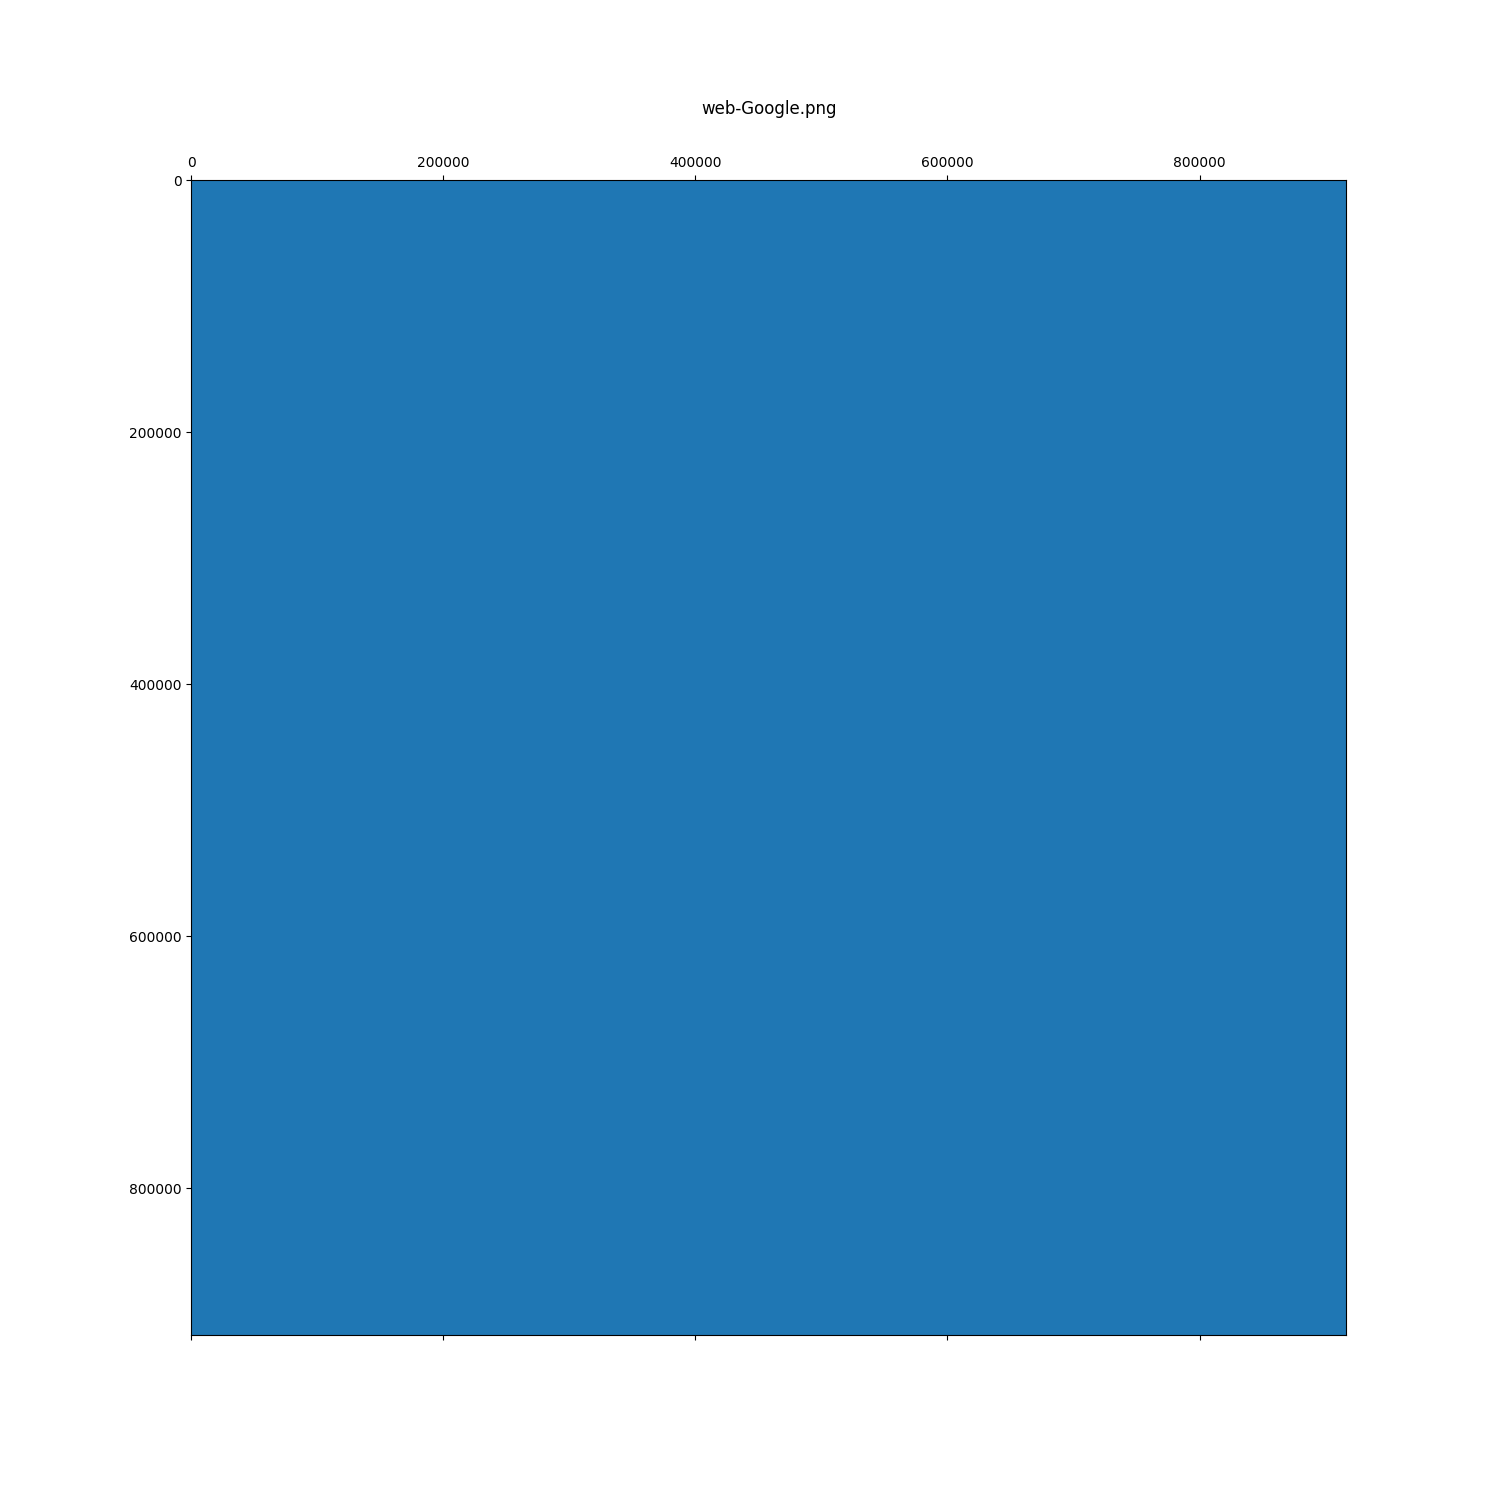}  \\ \hline
    
    \textcolor{darkred}{ldoor}	 & \includegraphics[width=0.23\textwidth]{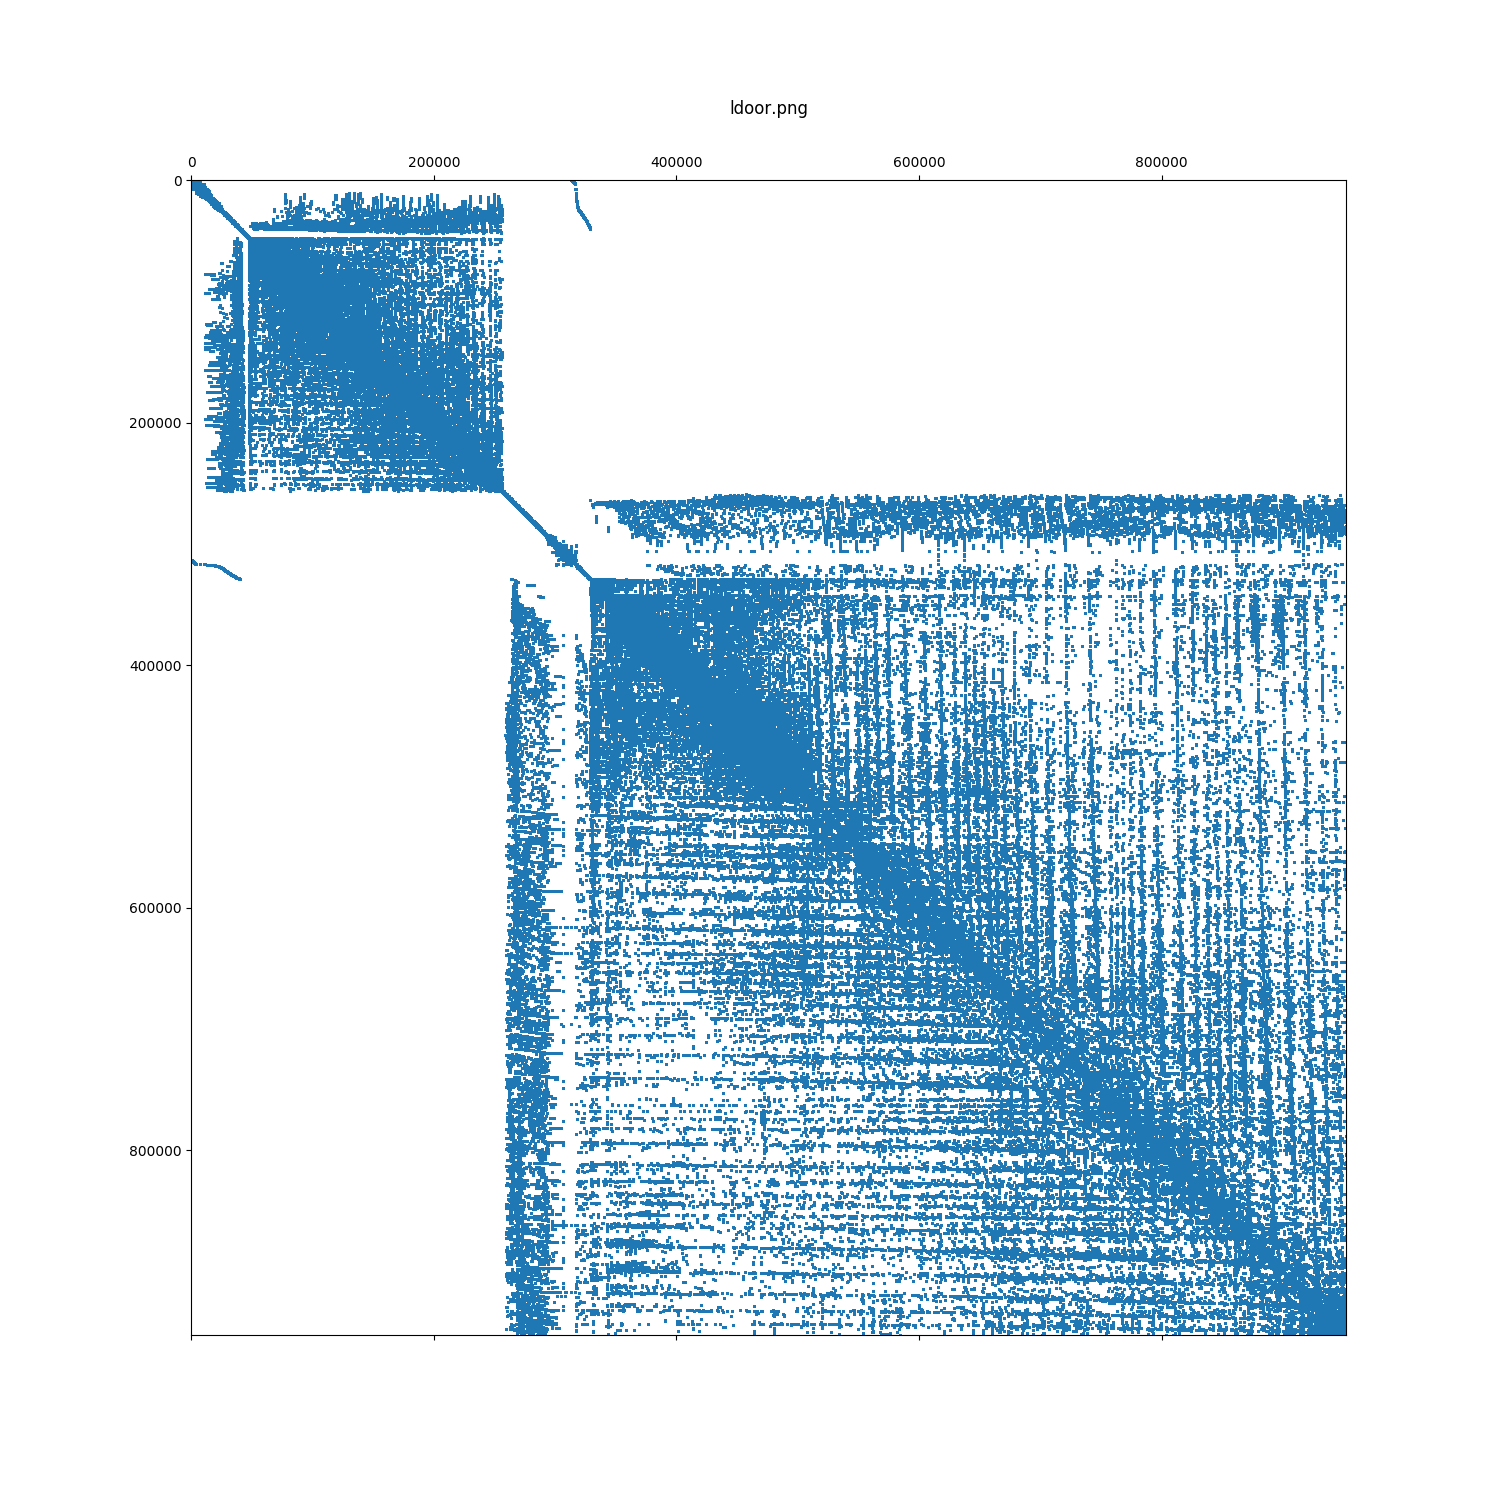}  \\ \hline 
    
    poisson3Db & \includegraphics[width=0.23\textwidth]{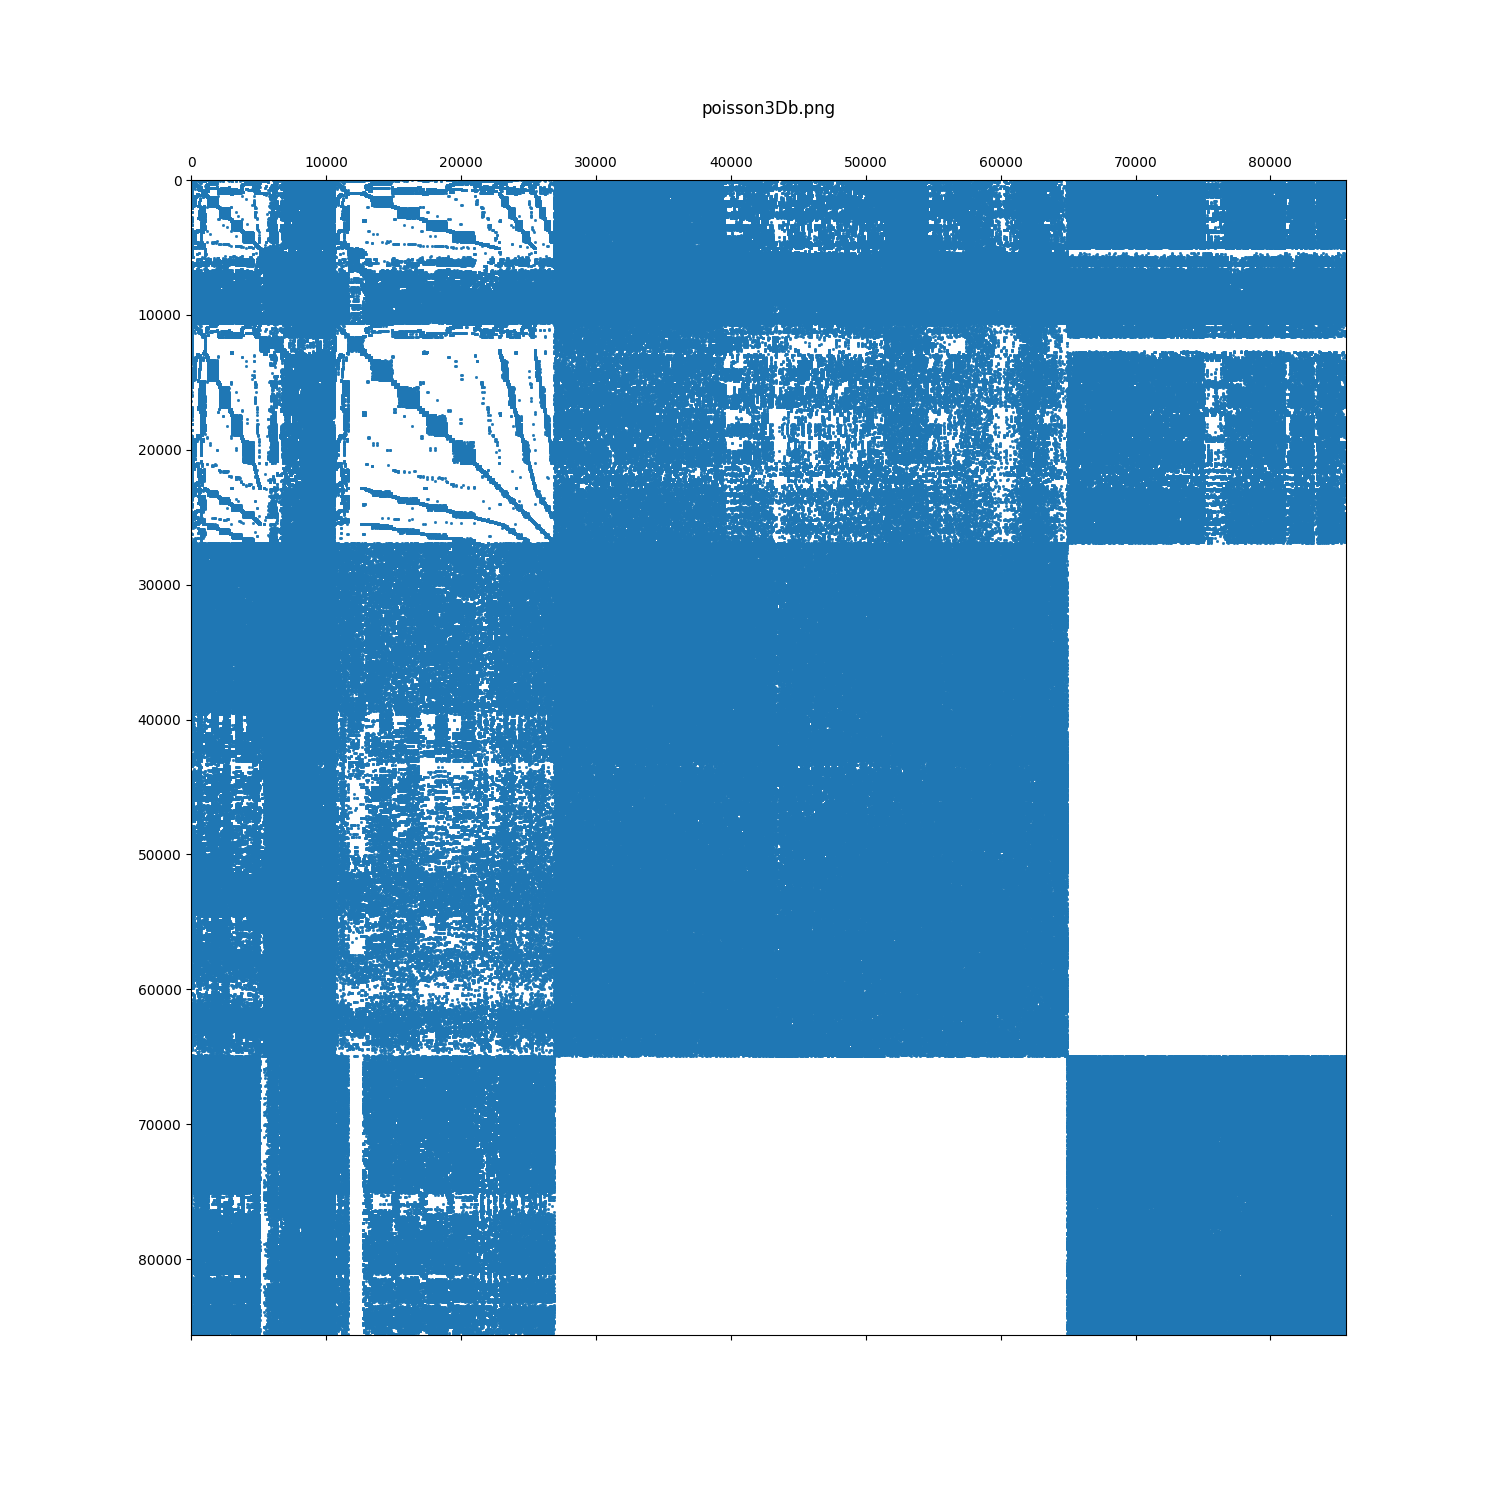}	 \\ \hline 
    
    \textcolor{darkred}{boneS10} & 	\includegraphics[width=0.23\textwidth]{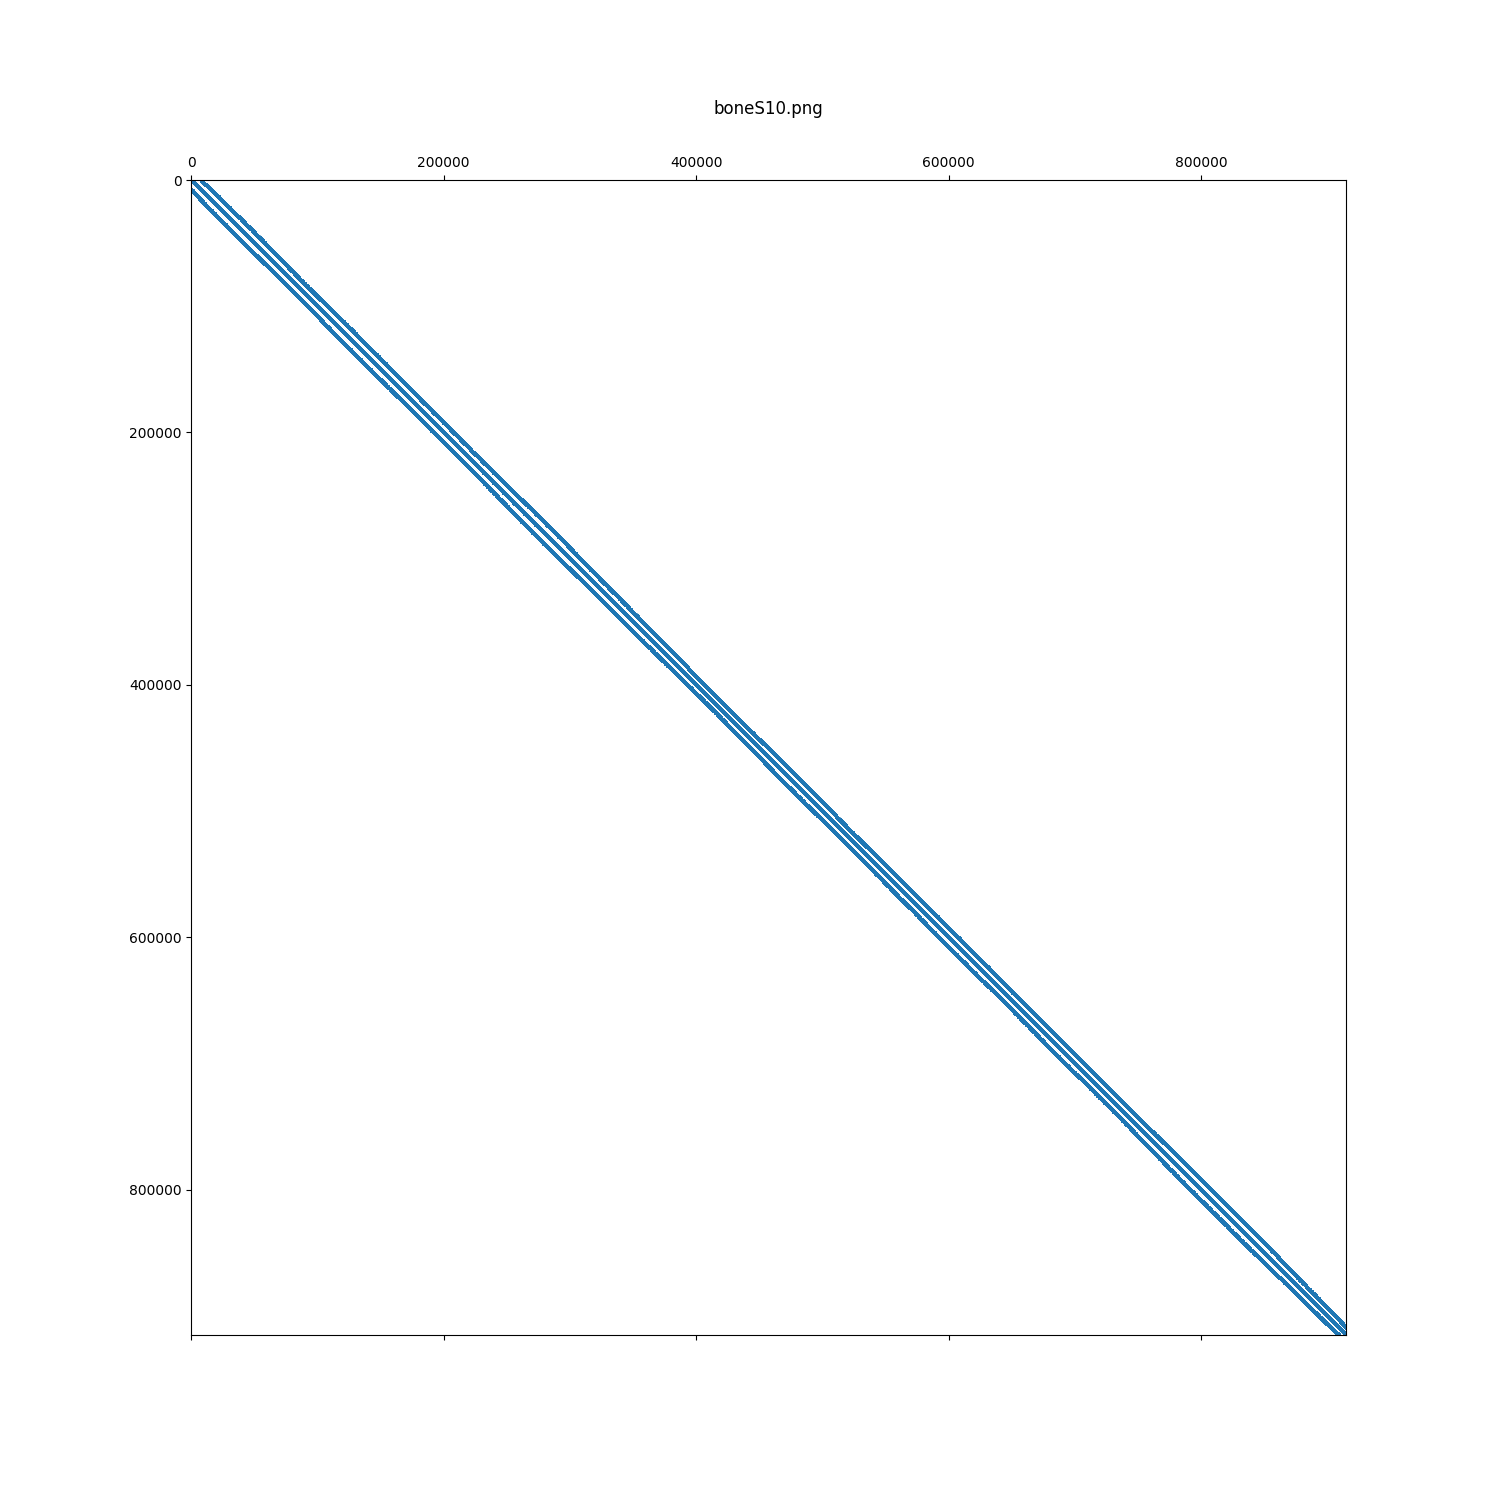}  \\ \hline 
    
    webbase-1M	& \includegraphics[width=0.23\textwidth]{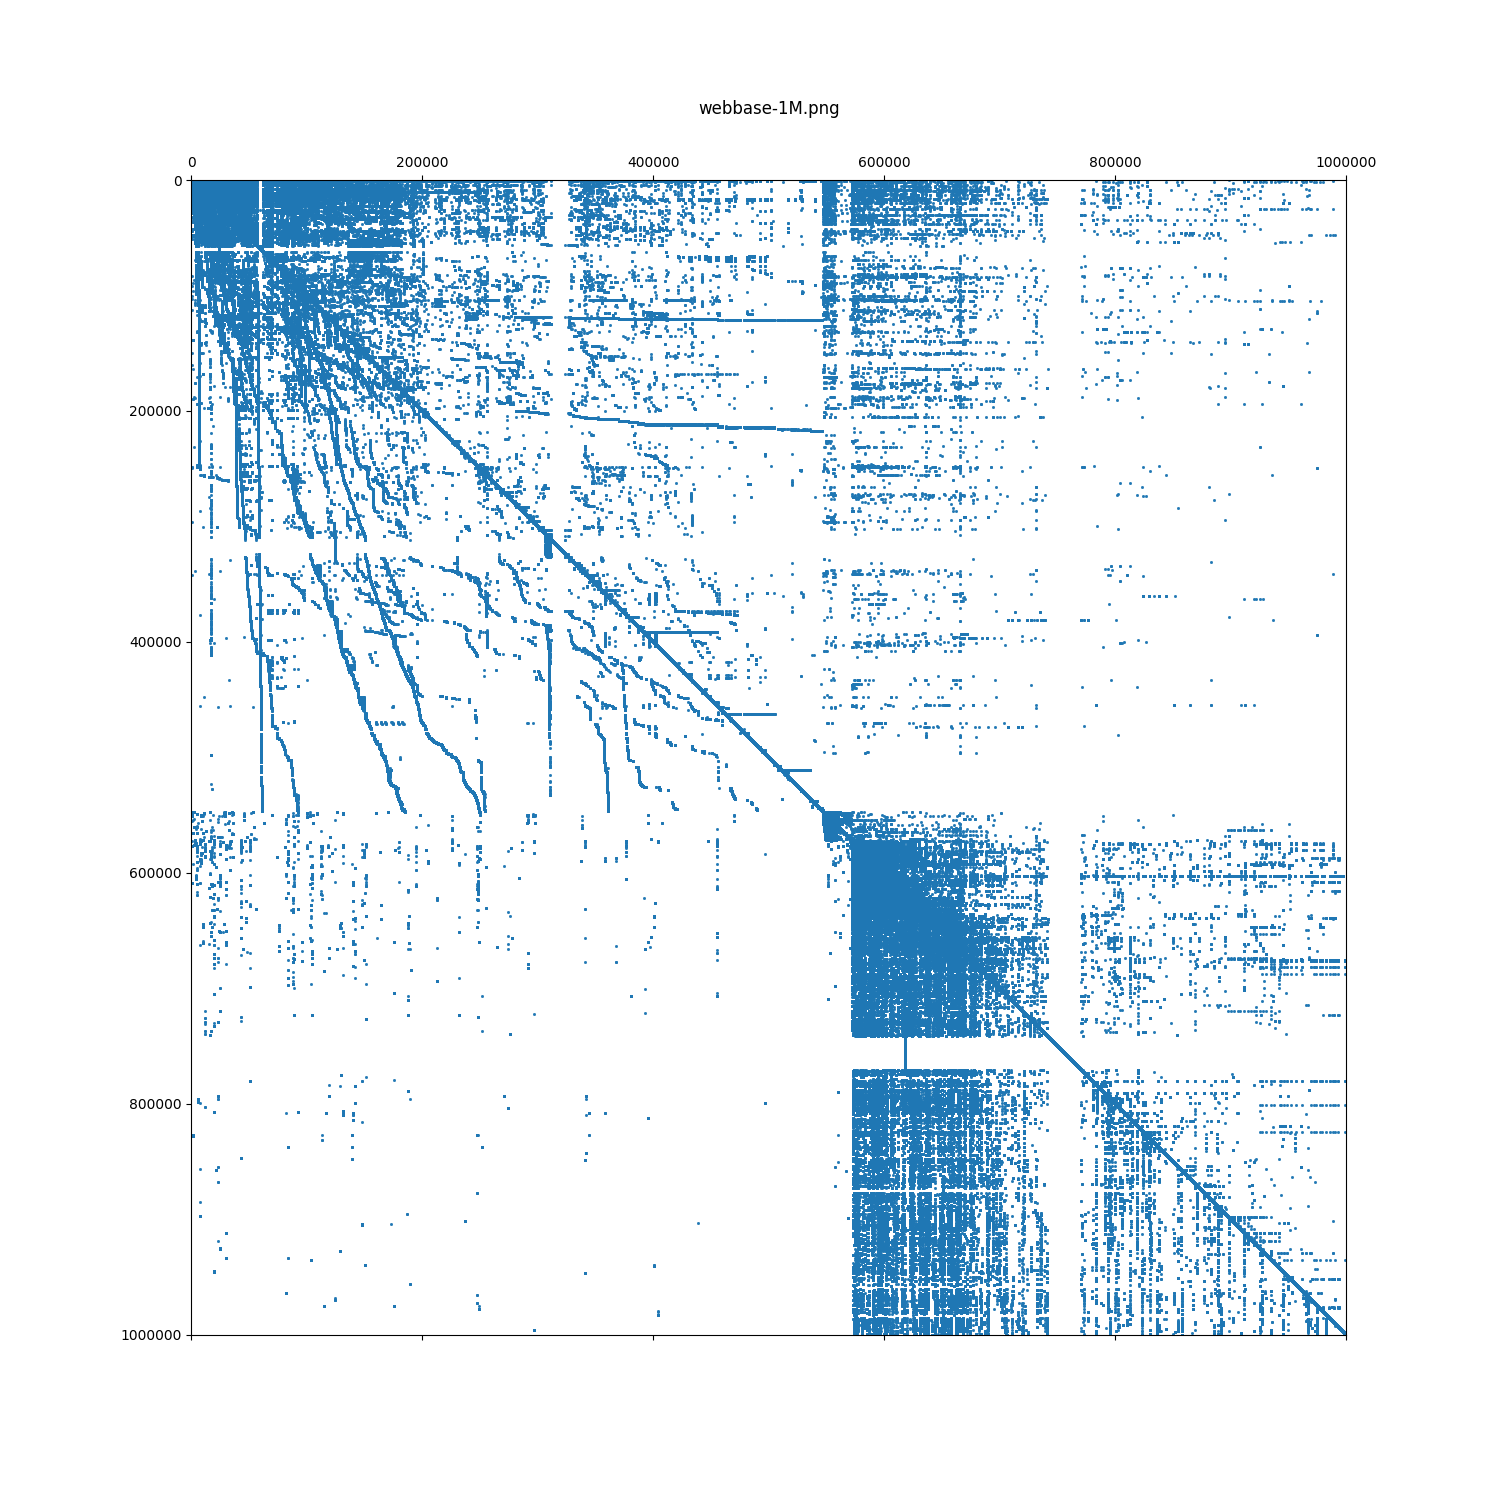} \\ \hline  
    
    in-2004 & \includegraphics[width=0.23\textwidth]{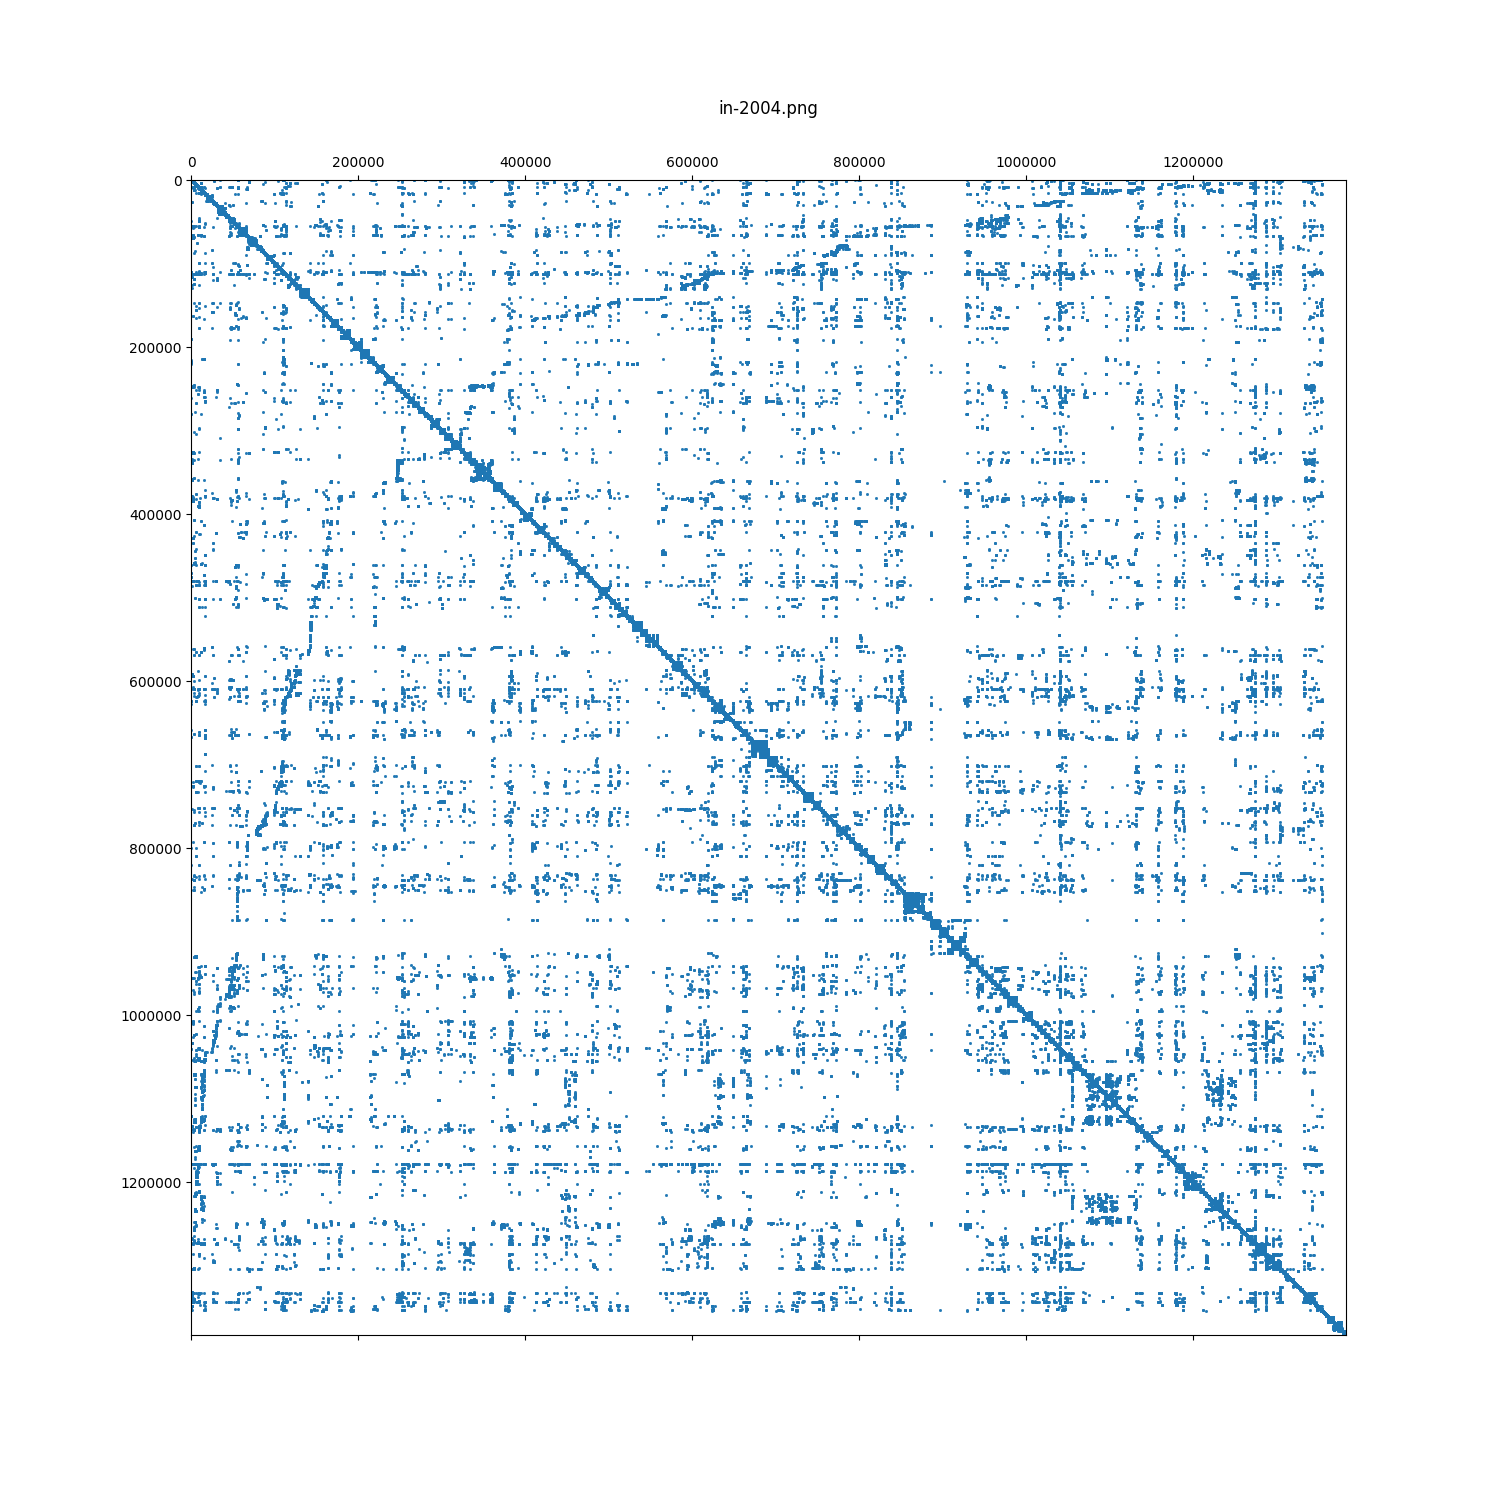} \\ \hline 
    
    \textcolor{darkred}{pkustk14} & \includegraphics[width=0.23\textwidth]{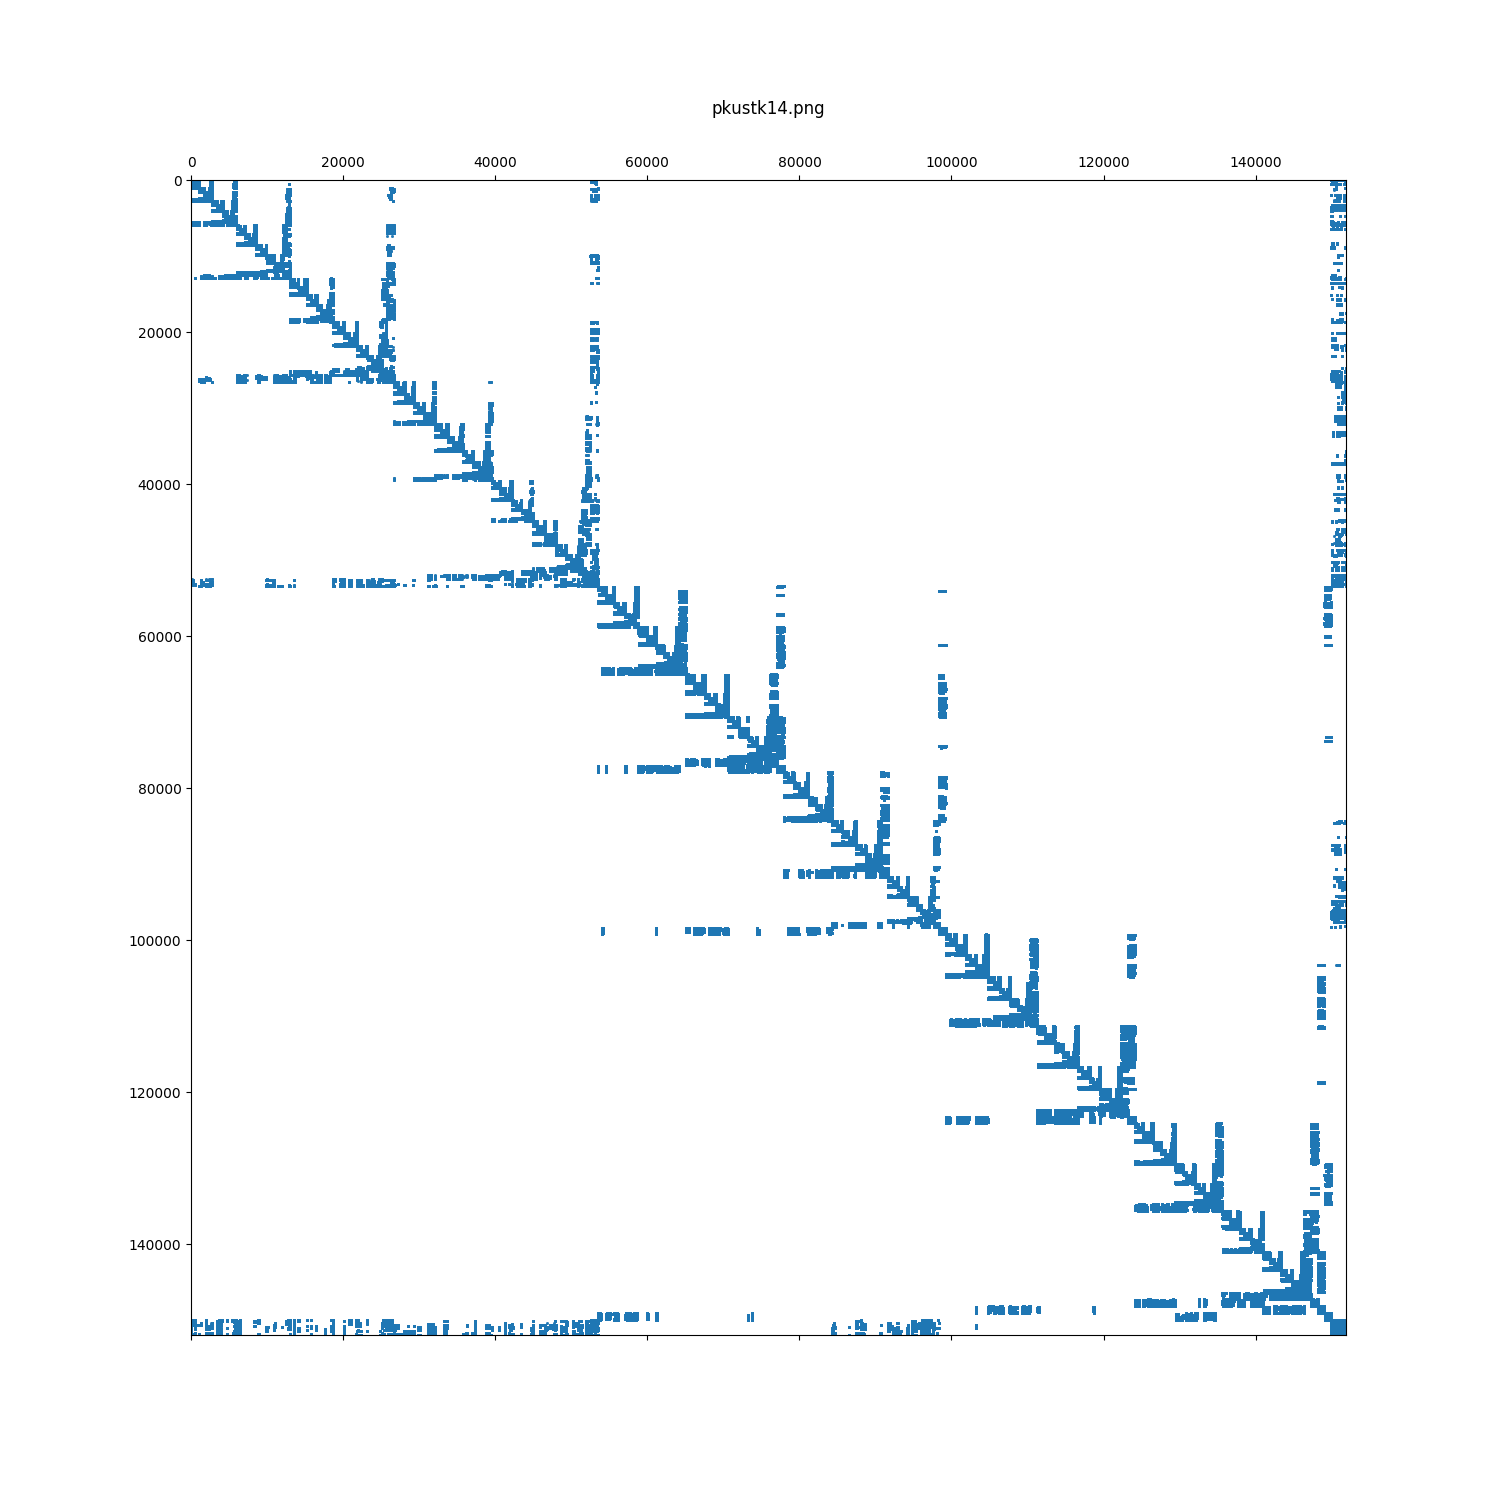}	\\ \hline  
    
    com-Youtube & \includegraphics[width=0.23\textwidth]{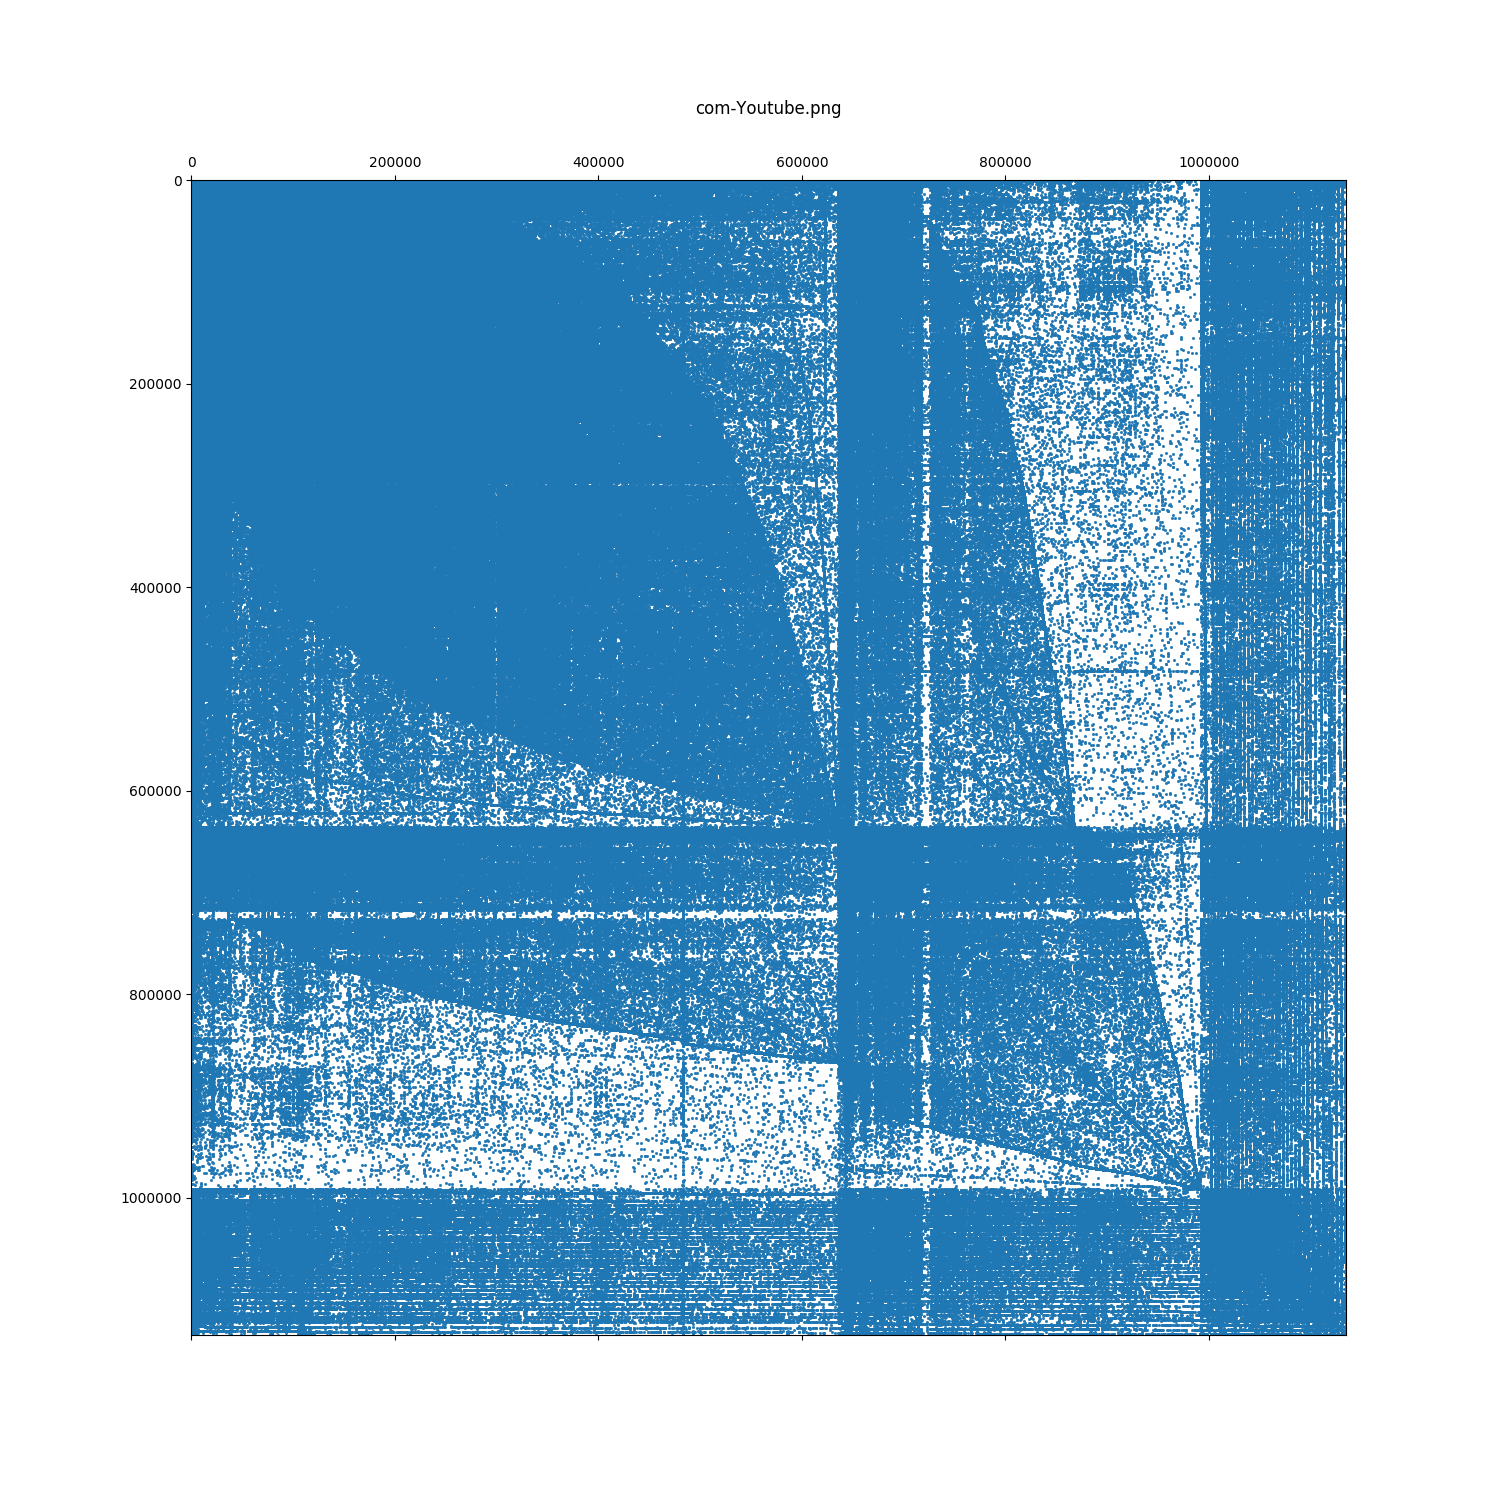} \\ \hline 

    
    sx-stackoverflow & \includegraphics[width=0.23\textwidth]{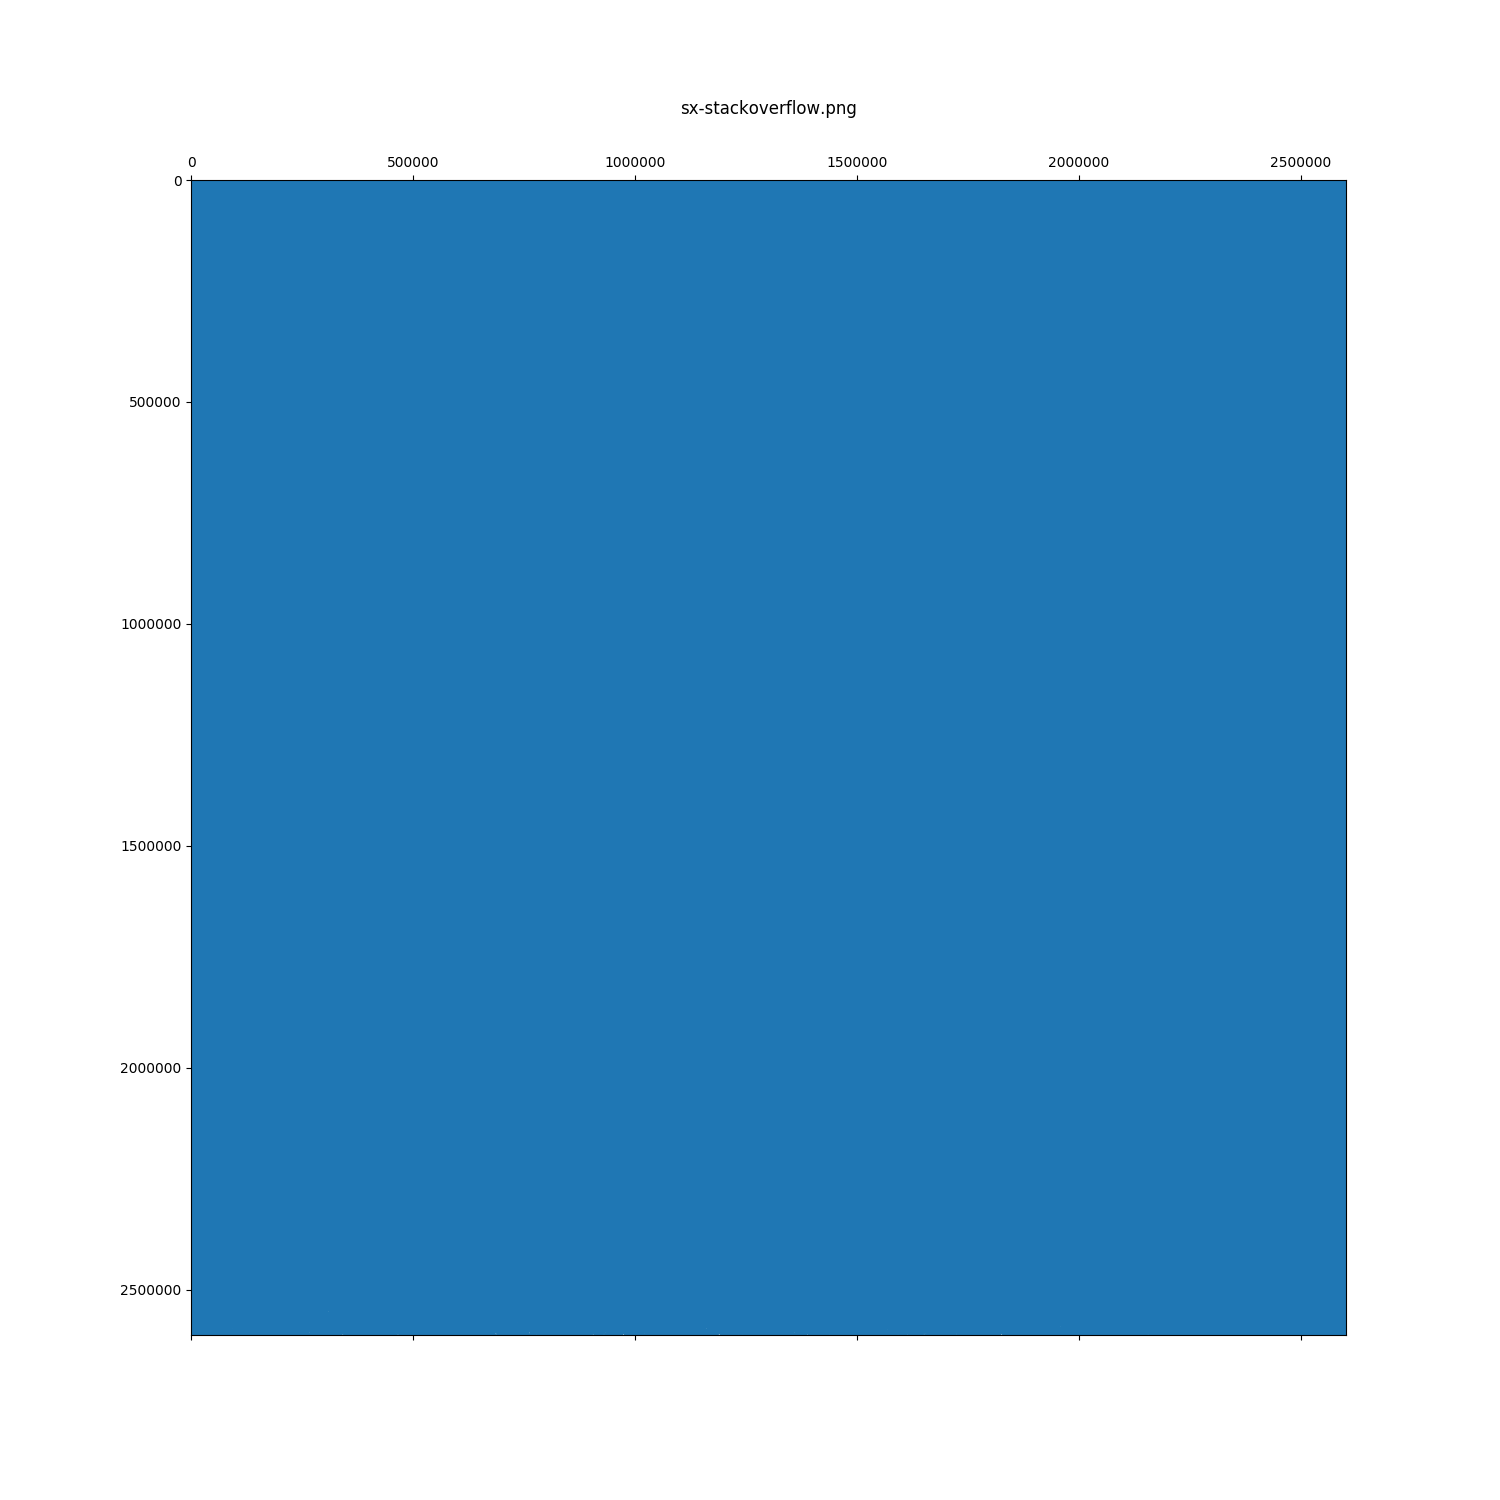} \\ \hline 
    
    as-Skitter & \includegraphics[width=0.23\textwidth]{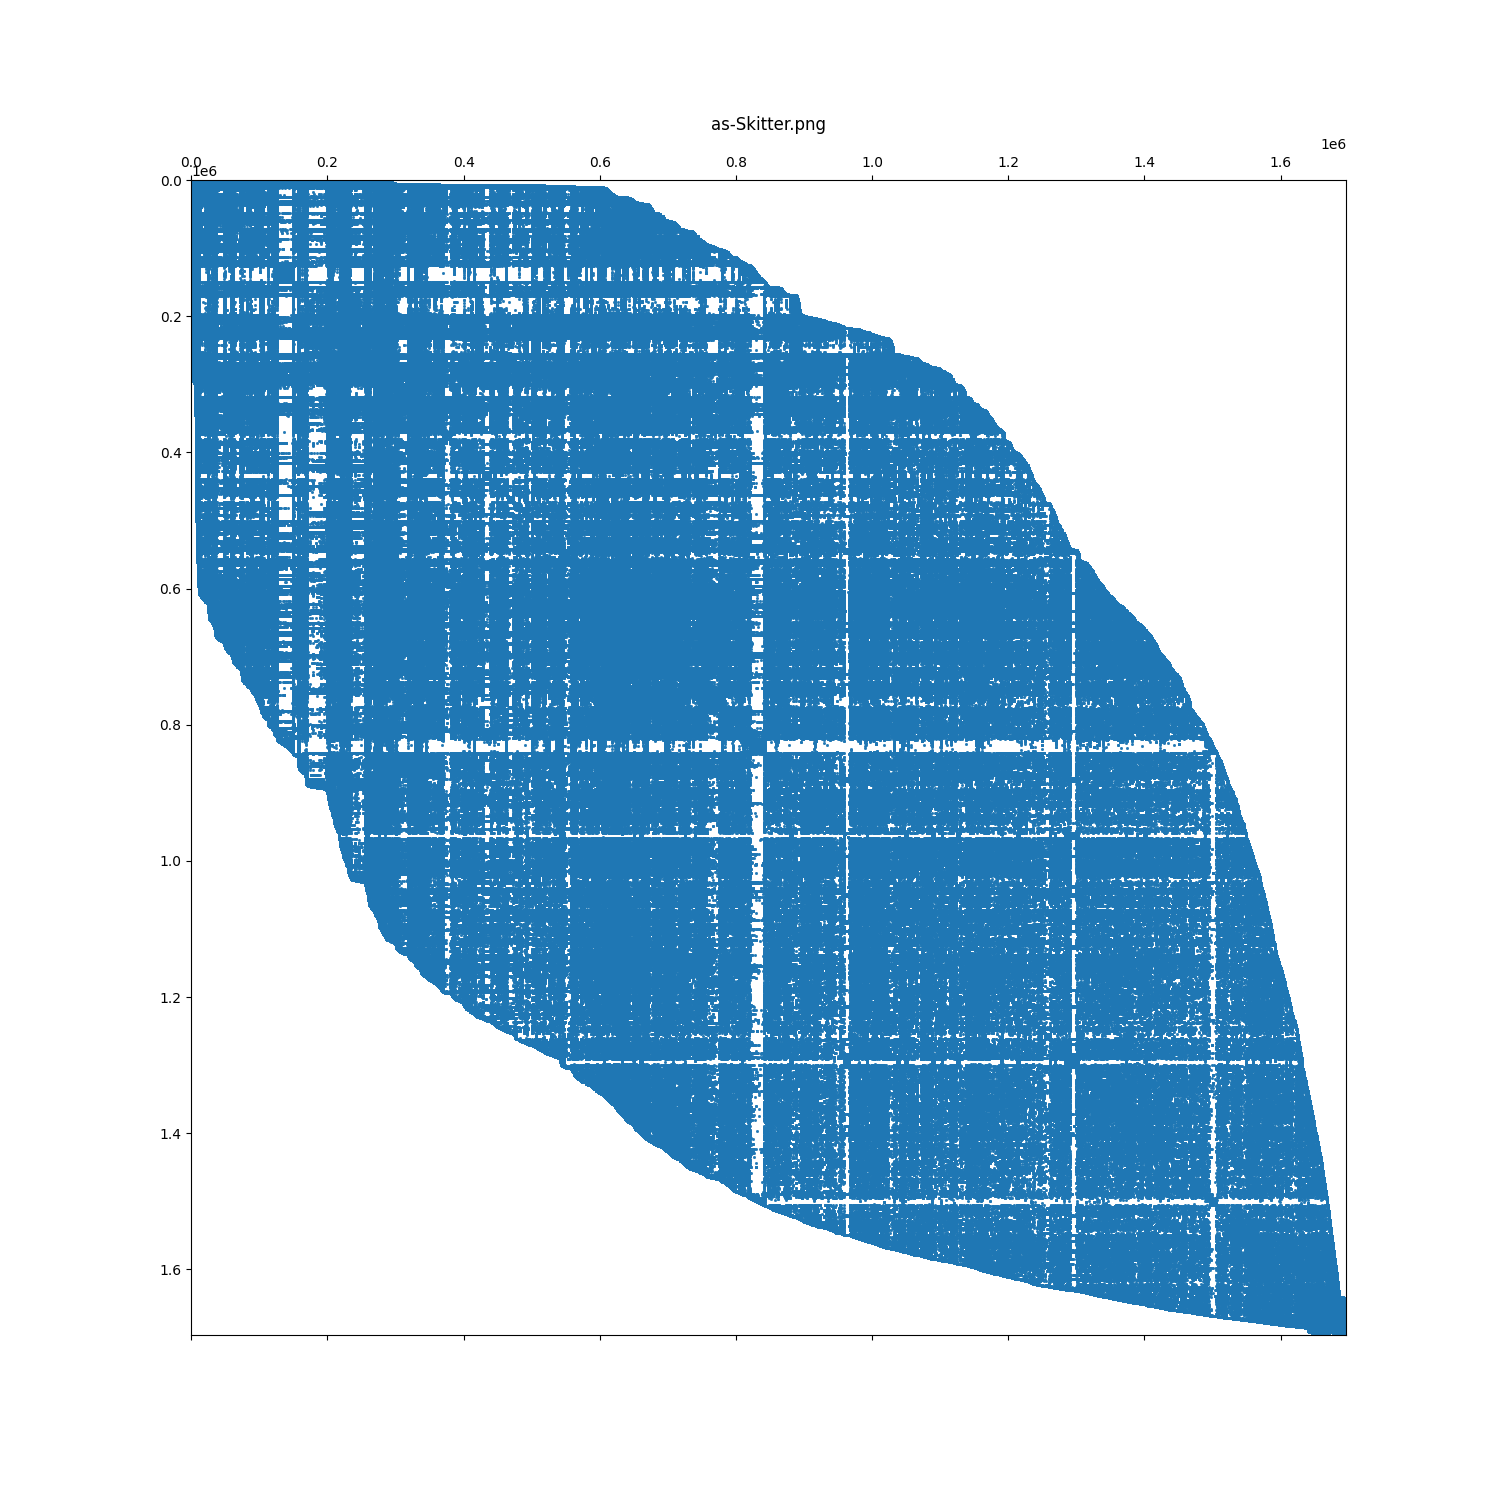} \\ \hline 
    
    ASIC\_680 & \includegraphics[width=0.23\textwidth]{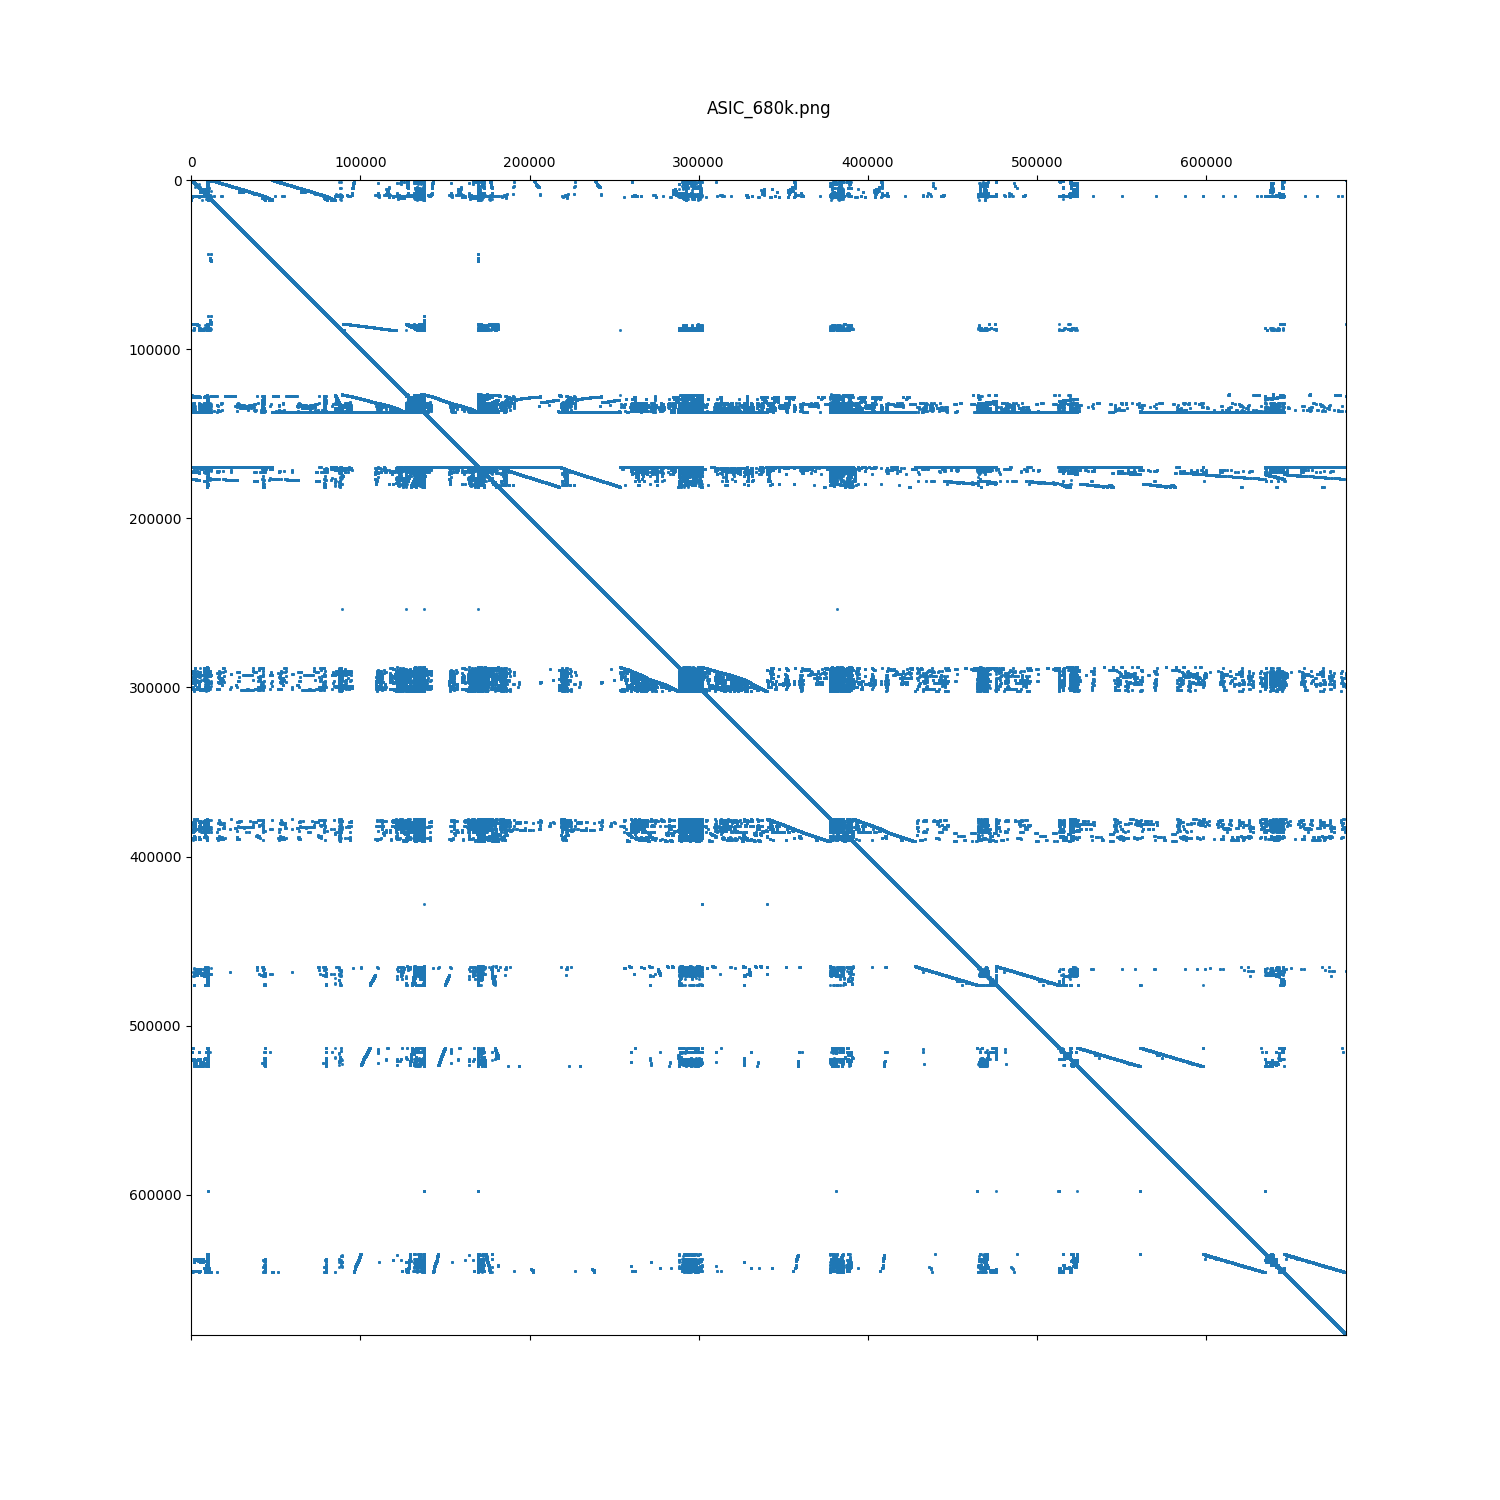} \\ \hline 
 
    \bottomrule
\end{tabular}
%}
\end{minipage}%
\end{center}
\caption{Graph plots for all matrices in our large matrix data set.}
\label{tab:appendix-large-matrices-plot}
\vspace{-8pt}
\end{table}


\section{Analysis of \spmv{} in Two Different UpMEM-based PIM Systems}

\arxiv{Table~\ref{tab:pim-systems} shows the characteristics of two UPMEM-based PIM systems. We calculate the available peak performance and memory bandwidth assuming 2048 DPUs in both PIM systems. In this section, we compare the \spmv{} execution in two different UPMEM-based PIM sytems using 2048 DPUs and 16 tasklets.}

\begin{table}[H]
\begin{center}
\centering
\resizebox{1.0\linewidth}{0.04\textheight}{
\begin{tabular}{lcccccccc}
    \toprule
    \textbf{System}  & \textbf{Avail. DPUs} & \textbf{Frequency} & \textbf{PIM Peak Performance} & \textbf{PIM Bandwidth} & \textbf{Host CPU} & \textbf{Host Peak Performance} & \textbf{Bus Bandwidth}  \\
    \midrule
    PIM System A & 2048 DPUs & 350 MHz & 3.78 GFLOPS & 1.43 TB/s &  Intel Xeon Silver 4110 @2.1GHz & 660 GFLOPS & 23.1 GB/s\\ \hline 
    PIM System B & 2048 DPUs & 425 MHz & 4.63 GFLOPS & 1.74 TB/s &  Intel Xeon Silver 4125 @2.5GHz & 1016 GFLOPS & 21.8 GB/s \\ \hline 
    \bottomrule
\end{tabular}
}
\end{center}
\caption{Evaluated UPMEM PIM Systems.}
\label{tab:pim-systems}
\end{table}



\arxiv{Figures~\ref{fig:cloud4-cloud7_fixed_vertpartitions}, ~\ref{fig:cloud4-cloud7_rbal_vertpartitions} and ~\ref{fig:cloud4-cloud7_bal_vertpartitions} compare the performance achieved using two different UPMEM-based PIM systems in 2D partitioning techniques with COO format, when varying the number of vertical partitions from 1 to 32, and having 2048 DPUs for int32 (left) and dbl64 (right) data types. We observe that the number of vertical partitions which provides the best performance on \spmv{} execution depends on the characteristics of the underlying hardware. For example, in PIM system B and int32 data type, the best-performing \spmv{} execution of DCOO using hgc matrix is achieved with 16 vertical partitions, while in PIM system A the best-performing execution of DCOO is achieved with 8 vertical partitions. Similarly, in PIM system A and dbl64 data type, the best-performing \spmv{} execution of BDCOO on the rjt matrix is achieved using 4 vertical partitions. However, in PIM system B and dbl64 data type, the performance of BDCOO on the rjt matrix does not improves when having more than 1 vertical partition, i.e., the \variableSized{} 2D partitioning scheme does not improve performance over the 1D partitioning scheme (1 vertical partition). Overall, based on our analysis we conclude that the parallelization scheme that achieves the best performance in \spmv{} depends on the hardware characteristics of the PIM system.}


\begin{figure}[H]
    \centering
    \begin{minipage}{\textwidth}
    \centering
    \includegraphics[width=.49\textwidth]{2D-partitioning/cloud4_cloud7_fixed_vertical_dpus2048_int32.pdf}
    \includegraphics[width=.49\textwidth]{2D-partitioning/cloud4_cloud7_fixed_vertical_dpus2048_dbl64.pdf}
    \end{minipage}
    \vspace{-10pt}
    \caption{Time breakdown of dcoo format and 2048 DPUs when varying the number of vertical partitions from 1 to 32 for int32 (left) and dbl64 (right) data types on two different configurations of UPMEM-based PIM systems.}
    \label{fig:cloud4-cloud7_fixed_vertpartitions}
\end{figure}


\begin{figure}[H]
    \centering
    \begin{minipage}{\textwidth}
    \centering
    \includegraphics[width=.49\textwidth]{2D-partitioning/cloud4_cloud7_rbal_vertical_dpus2048_int32.pdf}
    \includegraphics[width=.49\textwidth]{2D-partitioning/cloud4_cloud7_rbal_vertical_dpus2048_dbl64.pdf}
    \end{minipage}
    \vspace{-10pt}
    \caption{Time breakdown of rbdcoo format and 2048 DPUs when varying the number of vertical partitions from 1 to 32 for int32 (left) and dbl64 (right) data types on two different configurations of UPMEM-based PIM systems.}
    \label{fig:cloud4-cloud7_rbal_vertpartitions}
\end{figure}



\begin{figure}[H]
    \centering
    \begin{minipage}{\textwidth}
    \centering
    \includegraphics[width=.49\textwidth]{2D-partitioning/cloud4_cloud7_bal_vertical_dpus2048_int32.pdf}
    \includegraphics[width=.49\textwidth]{2D-partitioning/cloud4_cloud7_bal_vertical_dpus2048_dbl64.pdf}
    \end{minipage}
    \vspace{-10pt}
    \caption{Time breakdown of bdcoo format and 2048 DPUs when varying the number of vertical partitions from 1 to 32 for int32 (left) and dbl64 (right) data types on two different configurations of UPMEM-based PIM systems.}
    \label{fig:cloud4-cloud7_bal_vertpartitions}
\end{figure}



\arxiv{
Figure~\ref{fig:cloud4-cloud7} compares the performance of 1D and 2D partitioning techniques in two different UPMEM-based PIM systems (Table~\ref{tab:pim-systems}). For 1D partitioning, we use the lock-free COO and lock-based BCOO kernels. For each matrix, we vary the number of DPUs from 64 to 2048 DPUs, and select the best-performing execution. For 2D partitioning, we use the \equallySized{} COO and BCOO kernels using 2048 DPUs in both systems. For each matrix, we vary the number of vertical partitions from 2 to 32 (step of power of 2), and select the best-performing execution. 
}


\begin{figure}[H]
    %\vspace{-1pt}
    \centering
    \includegraphics[width=.999\textwidth]{2D-partitioning/cloud4_cloud7_simple_dpus2048_flt32.pdf}
    \vspace{-10pt}
    \caption{Throughput achieved by 1D and 2D partitioning techniques for flt32 data type using two different configurations of UPMEM-based PIM systems.}
    \label{fig:cloud4-cloud7}
\end{figure}



\arxiv{We draw out three findings. First, in both systems the best performance is achieved using a much smaller number of DPUs than 2048 DPUs (much smaller than the available DPUs on the system). This is because in both 1D and 2D partitioning kernels the \spmv{} execution is significantly bottlenecked by the expensive data transfer costs performed via the narrow memory bus, thus algorithms that fully exploit all available DPUs of the system incur high performance overheads in data transfers. Second, in both systems 2D partitioning kernels outperform the 1D partitioning kernels in relatively regular matrices, while 1D partitioning kernels perform better in scale-free matrices, i.e., in matrices with high non-zero element deviation among rows and columns. Third, we observe that PIM system (B) improves performance over PIM system (A) by 1.14$\times$ on average, because its DPUs included run at a higher frequency (425MHz vs 350MHz), thus providing higher peak system performance. Specifically, assuming 2048DPUs, peak throughput of PIM system A and PIM system B is 3.78 GFlops and 4.63 GFlops, respectively, i.e., PIM system B provides 1.22 $\times$ higher throughput.}
